# Supplementary material for: High-Dimensional Differential Parameter Inference in Exponential Family using Time Score Matching
Source: arXiv:2410.10637 source file (2025-04-05)
Supplement: Supplementary file 1 [file appendix.tex]

\subsection{\texorpdfstring{Asymptotic Distribution of $\partial_t \widehat{\boldsymbol{\theta}}_t$}{Asymptotic Distribution of partial_t theta_t}}

{\color{red} to be revised}

Consider a null hypothesis: the time series is stationary, i.e., $\partialthetastarsmall = \mb{0}$.  The alternative hypothesis corresponds to a change happening at time $t$, i.e., $\partialthetastarsmall \neq \mb{0}$. The following theorem allows us to quantify the asymptotic null distribution of $\partialthetahatsmall$ under this null hypothesis.
\begin{theorem}
 Let \cref{ass:alphastar} hold, and let $\widehat{\mb\alpha}$ be a minimiser of \cref{eq:sampleobj}, and $\partialthetahatsmall = \modeldthetahat$. As $n \to \infty$ and $T \to \infty$, the asymptotic distribution of $\partialthetahatsmall$ under the null hypothesis that $\partialthetastarsmall = \mb{0}$ is given by
\[
\partialthetahatsmall \sim  \mathcal{N}\br{0, \mb\Sigma_{\partialthetahatsmall}},
\]
where
\begin{align*}
\mb\Sigma_{\partialthetahatsmall} &= (\partial_t \mb\phi(t))^\top \mb\Sigma_A^{-1}  \mb\Sigma_B \mb\Sigma_A^{-1}(\partial_t \mb\phi(t)), \\
    \mb\Sigma_A &\coloneqq 
\sum^T_{j=1}\Eqtsmall\brs{\nabla_{\mb\alpha}^2 \mb{m}_{\mb\alpha}(\mb{x}, t_j)\big\vert_{\mb\alpha = \mb\alpha^\star}}, \\
    \mb\Sigma_B &\coloneqq  \sum^T_{j=1}
\mathrm{Var}\brs{\nabla_{\mb\alpha} \mb{m}_{\mb\alpha}(\mb{x}, t_j)\big\vert_{\mb\alpha = \mb\alpha^\star}},
\end{align*}
and
\begin{align*}
\nabla_{\mb\alpha} \mb{m}_{\mb\alpha^\star} &\coloneqq 
2 \brangle{ \partial_t g_t(\partial_t \mb\phi_t)^\top + g_t (\partial_t^2 \mb\phi_t)^\top, \mb{f}} \\
\nabla_{\mb\alpha}^2 \mb{m}_{\mb\alpha^\star} &\coloneqq 
2 g_t (\mb{f} - \Eqtsmall [\mb{f}]) (\mb{f} - \Eqtsmall [\mb{f}])^\top (\partial_t \mb\phi_t)(\partial_t \mb\phi_t)^\top
\end{align*}
are the first and second derivatives of $m_{\mb\alpha}$ evaluated at $\mb\alpha^\star$, and for brevity $\nabla_{\mb\alpha}\mb{m}_{\mb\alpha^\star} = \nabla_{\mb\alpha}\mb{m}_{\mb\alpha}(\mb{x}, t)\vert_{\mb\alpha = \mb\alpha^\star}$, 
$\nabla_{\mb\alpha}^2\mb{m}_{\mb\alpha^\star} = \nabla_{\mb\alpha}^2\mb{m}_{\mb\alpha}(\mb{x}, t)\vert_{\mb\alpha = \mb\alpha^\star}$, $\mb{f} = \mb{f}(\mb{x})$ and $\mb\phi_t = \mb\phi(t)$. 
\label{thm:asymptotic}
\end{theorem}
For proof, see \cref{app:asymptotic}. The proof revolves around first finding the asymptotic distribution for $\widehat{\mb\alpha}$ and transforming it to determine the asymptotic distribution for $\partialthetahatsmall$. This asymptotic distribution is fully specified without requiring knowledge of $\mb\alpha^\star$, and allows us to quantify the variance of the estimator $\partialthetahatsmall$ under the null hypothesis.

\section{Proof of Theorem \ref{thm:score}} \label{app:scoret}

Recall that 
\[
q_t = q(\mb{x}; \mb\theta^\star_t, \mb\varphi^\star) = \frac{\exp \left(\brangle{\mb\theta^\star(t), \mb{f}(\mb{x})} + \brangle{
\mb\varphi^\star, \mb{h}(\mb{x})
}\right)
}{Z(\mb\theta^\star(t), \mb\varphi^\star)},
\]
where $\mb\varphi$ does not depend on $t$ and therefore $\partial_t \mb\varphi = 0$, and for simplicity we have written $\mb\theta_t = \mb\theta(t)$. Next,
\begin{align*}
     \scoret{q_t} = \partial_t \log q_t & = \partial_t \brs{\brangle{\mb\theta^\star_t, \mb{f}(\mb{x})} + \brangle{ \mb\varphi^\star, \mb{h}(\mb{x})}} - \partial_t \log Z(\mb\theta^\star_t, \mb\varphi^\star) \\
     &= \brangle{\partialthetastarsmall, \mb{f}(\mb{x})} - \frac{ \partial_t  Z(\mb\theta^\star_t, \mb\varphi^\star)}{Z(\mb\theta^\star_t, \mb\varphi^\star)} \\
     &= \brangle{\partialthetastarsmall, \mb{f}(\mb{x})}  - \frac{ \partial_t  \xintegral \exp \left(\brangle{\mb\theta^\star(t), \mb{f}(\mb{x})} + \brangle{
\mb\varphi^\star, \mb{h}(\mb{x})
}\right)d\mb{x} }{Z(\mb\theta^\star_t, \mb\varphi^\star)} \\
     &= \brangle{\partialthetastarsmall, \mb{f}(\mb{x})} - \frac{   \xintegral \partial_t \brs{\brangle{\mb\theta^\star(t), \mb{f}(\mb{x})} + \brangle{
\mb\varphi^\star, \mb{h}(\mb{x})
}}\exp \left(\brangle{\mb\theta^\star(t), \mb{f}(\mb{x})} + \brangle{
\mb\varphi^\star, \mb{h}(\mb{x})
}\right)d\mb{x}}{Z(\mb\theta^\star_t, \mb\varphi^\star)} \\
     &= \brangle{\partialthetastarsmall, \mb{f}(\mb{x})} - \frac{   \xintegral \brangle{\partialthetastarsmall, \mb{f}(\mb{x})}\exp \left(\brangle{\mb\theta^\star(t), \mb{f}(\mb{x})} + \brangle{
\mb\varphi^\star, \mb{h}(\mb{x})
}\right) d\mb{x} }{Z(\mb\theta^\star_t, \mb\varphi^\star)} \\
     &= \brangle{\partialthetastarsmall, \mb{f}(\mb{x})} -    \xintegral \brangle{\partialthetastarsmall, \mb{f}(\mb{x})}\frac{\exp \left(\brangle{\mb\theta^\star(t), \mb{f}(\mb{x})} + \brangle{
\mb\varphi^\star, \mb{h}(\mb{x})
}\right)}{Z(\mb\theta^\star_t, \mb\varphi^\star)}d\mb{x}  \\
     &= \brangle{\partialthetastarsmall, \mb{f}(\mb{x})} -    \xintegral \brangle{\partialthetastarsmall, \mb{f}(\mb{x})}q(\mb{x}; \mb\theta^\star_t, \mb\varphi^\star)d\mb{x} \\
     &= \brangle{\partialthetastarsmall, \mb{f}(\mb{x})} -    \Eqtsmall\brs{ \brangle{\partialthetastarsmall, \mb{f}(\mb{x})}},
\end{align*}
as desired. All equalities either come from applications of the chain rule or simple rearrangements.

\section{Proof of Example \ref{ex:gaussian_score}} \label{app:gaussian_score}

Let us group this example into three parts: fixed mean and time-dependent variance ($\mu$ and $\sigma_t^2$), time-dependent mean and fixed variance ($\mu_t$ and $\sigma^2$), and time-dependent mean and variance ($\mu_t$ and $\sigma_t^2$). Each one is detailed in distinct sections below.

Across all three cases we aim to verify the following equation holds 
\begin{equation}
\partial_t \log q_t = \langle \partialthetasmall, \mb{f}({x}) - \E_{q_t} [\mb{f}({x})] \rangle,
\label{eq:app:dlogqt}
\end{equation}
which is our formulation given by \cref{thm:score}. For the exponential family, the natural parameterisation of the Gaussian distribution is given by
\begin{equation}
\mb\theta = \begin{bmatrix}
    \frac{\mu}{\sigma^2} \\ -\frac{1}{2\sigma^2}
\end{bmatrix}
\label{eq:app:naturalparams}
\end{equation}
for a given $\mu$ and $\sigma^2$.

\paragraph{Fixed mean and time-dependent variance} 

Let the fixed mean be written as $\mu$ and the time-dependent variance be written as $\sigma_t^2$. 
Firstly, according to this Gaussian distribution, the LHS of \cref{eq:app:dlogqt} is given by
\begin{align}
\partial_t \log q_t &= \partial_t \br{\frac{-(x-\mu)^2}{2\sigma_t^2}} - \partial_t \log (\sqrt{2\pi}\sigma_t) \nonumber \\
&= - \partial_t \br{\frac{x^2}{2\sigma_t^2}} + \partial_t\br{\frac{x\mu}{\sigma_t}} - \partial_t\br{\frac{\mu^2}{2\sigma_t^2}} - \partial_t \br{\log \sigma_t} \nonumber \\
&= - x^2 \partial_t \br{\frac{1}{2\sigma_t^2}} + x\mu \partial_t\br{\frac{1}{\sigma_t}} - \mu^2 \partial_t\br{\frac{1}{2\sigma_t^2}} - \frac{\partial_t \sigma_t}{\sigma_t} \label{eq:app:fixed_mean_time_var}
\end{align}
We aim to show that when $\mb{f}(x) = [x, x^2]$, the RHS of \cref{eq:app:dlogqt} is equal to this. We first write
\[
\mb\theta_t = \begin{bmatrix}
    \frac{\mu}{\sigma_t^2} \\ -\frac{1}{2\sigma_t^2}
\end{bmatrix}, \qquad \partialthetasmall = \begin{bmatrix}
    \mu \partial_t \br{\frac{1}{\sigma_t^2}} \\ -\partial_t \br{\frac{1}{2\sigma_t^2}}
\end{bmatrix}.
\]
\begin{align*}
    \left\langle \partial_t \theta_t, \mb{f}({x}) - \E_{q_t} [\mb{f}({x})] \right\rangle &= \left\langle \begin{bmatrix}
        \partial_t \br{ \frac{\mu}{\sigma_t^2} } \\
        \partial_t \br{ -\frac{1}{2\sigma_t^2} }         
    \end{bmatrix}, \begin{bmatrix}
        x \\
        x^2 
    \end{bmatrix} - \begin{bmatrix}
        \Eqtsmall[x] \\
        \Eqtsmall[x^2] 
    \end{bmatrix} \right\rangle \\
    &= \left\langle \begin{bmatrix}
        \partial_t \br{ \frac{\mu}{\sigma_t^2} } \\
        \partial_t \br{ -\frac{1}{2\sigma_t^2} }         
    \end{bmatrix}, \begin{bmatrix}
        x \\
        x^2 
    \end{bmatrix} - \begin{bmatrix}
        \mu \\
        \sigma_t^2 + \mu^2 
    \end{bmatrix} \right\rangle \\
    &= \left\langle \begin{bmatrix}
        \partial_t \br{ \frac{\mu}{\sigma_t^2} } \\
        \partial_t \br{ -\frac{1}{2\sigma_t^2} }         
    \end{bmatrix}, \begin{bmatrix}
        x - \mu \\
        x^2 - \sigma_t^2 - \mu^2
    \end{bmatrix}\right\rangle \\
    &= \partial_t \br{ \frac{\mu}{\sigma_t^2} } (x - \mu) - \partial_t \br{\frac{1}{2\sigma_t^2} }(x^2 - \sigma_t^2 - \mu^2) \\
    &=x\mu \partial_t\br{ \frac{1}{\sigma_t^2} } - \mu^2 \partial_t\br{ \frac{1}{\sigma_t^2} } - x^2\partial_t\br{ \frac{1}{2\sigma_t^2} } + \sigma_t^2 \partial_t\br{ \frac{1}{2\sigma_t^2} } + \mu^2 \partial_t\br{ \frac{1}{2\sigma_t^2} } \\
    &=x\mu \partial_t\br{ \frac{1}{\sigma_t^2} } - \mu^2 \partial_t\br{ \frac{1}{2\sigma_t^2} } - x^2\partial_t\br{ \frac{1}{2\sigma_t^2} } + \sigma_t^2 \partial_t\br{ \frac{1}{2\sigma_t^2} }. 
\end{align*}
By the chain rule,
\[
\sigma_t^2\partial_t\br{\frac{1}{2\sigma_t^2}} = \frac{\sigma_t^2}{2}\partial_t\br{\sigma_t^{-2}} = -\frac{\sigma_t^2}{2} \frac{2}{\sigma_t^3}\partial_t \sigma_t = -\frac{\partial_t \sigma_t}{\sigma_t},
\]
which, substituted into the equation above, leaves
\[
x\mu \partial_t\br{ \frac{1}{\sigma_t^2} } - \mu^2 \partial_t\br{ \frac{1}{2\sigma_t^2} } - x^2\partial_t\br{ \frac{1}{2\sigma_t^2} } - \frac{\partial_t\sigma_t}{\sigma_t}
\]
for which all terms match the terms in \cref{eq:app:fixed_mean_time_var} as desired.

Since we are doing very similar operations across all examples, the following two derivations will be lighter on details but should be straightforward to follow.

\paragraph{Time-dependent mean and fixed variance}
Firstly, write $\mu_t$ and $\sigma^2$ as the mean and variance of this Gaussian distribution, respectively. The time score function, i.e. the LHS of \cref{eq:app:dlogqt} is given by
\begin{align}
    \partial_t \log q_t &= \partial_t \br{\frac{-(x-\mu_t)^2}{2\sigma^2}} - \partial_t \log (\sqrt{2\pi}\sigma) \nonumber \\
&= \frac{2x \partial_t \mu_t - \partial_t (\mu_t^2)}{2\sigma^2} .\label{eq:app:dlogqt_time_mean_fixed_var}
\end{align}
The natural parameters are given by
\[
\mb\theta_t = \begin{bmatrix}
    \frac{\mu_t}{\sigma^2} \\ -\frac{1}{2\sigma^2}
\end{bmatrix}, \qquad \partialthetasmall = \begin{bmatrix}
    \partial_t \br{\frac{\mu_t}{\sigma^2}} \\ \partial_t \br{-\frac{1}{2\sigma^2}}
\end{bmatrix} = \begin{bmatrix}
    \frac{\partial_t \mu_t}{\sigma^2} \\ 0
\end{bmatrix},
\]
and so we consider the first dimension only. The RHS of \cref{eq:app:dlogqt}, when $\mb{f}(x) = x$ is given by
\begin{align*}
    \left\langle \partial_t \theta_t, \mb{f}({x}) - \E_{q_t} [\mb{f}({x})] \right\rangle &= \brangle{ \frac{ \partial_t \mu_t}{\sigma^2}, x - \mu_t} \\
    &= \frac{x \partial_t \mu_t - \mu_t \partial_t \mu_t}{\sigma^2} \\
    &= \frac{x \partial_t \mu_t - \frac{\partial_t (\mu_t^2)}{2}}{\sigma^2} \\
    &= \frac{2x \partial_t \mu_t - \partial_t (\mu_t^2)}{2\sigma^2} 
\end{align*}
where the penultimate line is due to the chain rule. This matches \cref{eq:app:dlogqt_time_mean_fixed_var} as desired.

\paragraph{Time-dependent mean and variance}

Firstly, write $\mu_t$ and $\sigma_t^2$ as the mean and variance of this Gaussian distribution, respectively. The time score function, i.e. the LHS of \cref{eq:app:dlogqt} is given by
\begin{align}
    \partial_t \log q_t &= \partial_t \br{\frac{-(x-\mu_t)^2}{2\sigma_t^2}} - \partial_t \log (\sqrt{2\pi}\sigma_t) \nonumber \\
&= -x^2 \partial_t \br{\frac{1}{2\sigma_t^2}} + x\frac{\partial_t \mu_t}{\sigma_t^2} + x\mu_t \partial_t \br{\frac{1}{\sigma_t^2}} - \frac{\partial_t (\mu_t^2)}{2\sigma_t^2} - \mu_t^2\partial_t \br{\frac{1}{2\sigma_t^2}} - \frac{\partial_t \sigma_t}{\sigma_t}.
\label{eq:app:dlogqt_time_mean_time_var}
\end{align}
The natural parameters are given by
\[
\mb\theta_t = \begin{bmatrix}
    \frac{\mu_t}{\sigma_t^2} \\ -\frac{1}{2\sigma_t^2}
\end{bmatrix}, \qquad \partialthetasmall = \begin{bmatrix}
    \partial_t \br{\frac{\mu_t}{\sigma_t^2}} \\ \partial_t \br{-\frac{1}{2\sigma_t^2}}
\end{bmatrix} = \begin{bmatrix}
    \frac{\partial_t \mu_t}{\sigma_t^2} + \mu_t\partial_t \br{\frac{1}{\sigma_t^2}} \\ -\partial_t\br{\frac{1}{2\sigma_t^2}}
\end{bmatrix},
\]
The RHS of \cref{eq:app:dlogqt} when $\mb{f}(x) = [x, x^2]$ is given by
\begin{align*}
    \left\langle \partial_t \theta_t, \mb{f}({x}) - \E_{q_t} [\mb{f}({x})] \right\rangle &= \left\langle \begin{bmatrix}
        \frac{\partial_t \mu_t}{\sigma_t^2} + \mu_t\partial_t \br{\frac{1}{\sigma_t^2}} \\ -\partial_t\br{\frac{1}{2\sigma_t^2}}     
    \end{bmatrix}, \begin{bmatrix}
        x - \mu_t \\
        x^2 - \sigma_t^2 - \mu_t^2
    \end{bmatrix}\right\rangle \\
    &= \br{\frac{\partial_t \mu_t}{\sigma_t^2} + \mu_t\partial_t \br{\frac{1}{\sigma_t^2}}}( x - \mu_t) - \partial_t\br{\frac{1}{2\sigma_t^2}}( x^2 - \sigma_t^2 - \mu_t^2)\\
    &= x \frac{\partial_t \mu_t}{\sigma_t^2} + x\mu_t\partial_t \br{\frac{1}{\sigma_t^2}} - \mu_t\frac{\partial_t \mu_t}{\sigma_t^2}  - \mu_t^2\partial_t \br{\frac{1}{\sigma_t^2}} - x^2 \partial_t\br{\frac{1}{2\sigma_t^2}} + \sigma_t^2 \partial_t\br{\frac{1}{2\sigma_t^2}} + \mu_t^2 \partial_t\br{\frac{1}{2\sigma_t^2}} \\
    &= x \frac{\partial_t \mu_t}{\sigma_t^2} + x\mu_t\partial_t \br{\frac{1}{\sigma_t^2}} - \mu_t\frac{\partial_t \mu_t}{\sigma_t^2}  + \mu_t^2\partial_t \br{\frac{1}{2\sigma_t^2}} - x^2 \partial_t\br{\frac{1}{2\sigma_t^2}} + \sigma_t^2 \partial_t\br{\frac{1}{2\sigma_t^2}}\\
    &= x \frac{\partial_t \mu_t}{\sigma_t^2} + x\mu_t\partial_t \br{\frac{1}{\sigma_t^2}} - \mu_t\frac{\partial_t \mu_t}{\sigma_t^2}  + \mu_t^2\partial_t \br{\frac{1}{2\sigma_t^2}} - x^2 \partial_t\br{\frac{1}{2\sigma_t^2}} - \frac{\partial_t \sigma_t}{\sigma_t} \\
    &= x \frac{\partial_t \mu_t}{\sigma_t^2} + x\mu_t\partial_t \br{\frac{1}{\sigma_t^2}} - \frac{\partial_t (\mu_t^2)}{2\sigma_t^2}  - \mu_t^2\partial_t \br{\frac{1}{2\sigma_t^2}} - x^2 \partial_t\br{\frac{1}{2\sigma_t^2}} - \frac{\partial_t \sigma_t}{\sigma_t},
\end{align*}
where the last three equalities, in their respective order, are due to collecting like terms, the chain rule on the last term, and the chain rule again on the third term. This matches \cref{eq:app:dlogqt_time_mean_time_var}, completing the proof.

\section{Proof of \cref{thm:obj_model}} \label{app:SMderivation_1}

Let us begin from the initial formulation of our time based score matching objective with weight function $g_t = g(t)$ for which $g(0) = g(1) = 0$, i.e. $g(t) = 0$ at the edges of our time domain $t \in [0, 1]$. The initial objective is given by
\begin{align*}
\ourJ &= \timeintegral \Eqtsmall\brs{g_t \| \scoret{q_t} - \modelsmall \|^2} dt \\
     &= \timeintegral \Eqtsmall\brs{g_t \modelsmall^2} dt - 2 \timeintegral\Eqtsmall\brs{g_t \modelsmall \scoret{q_t}}dt + \timeintegral\Eqtsmall\brs{g_t\scoret{q_t}^2} dt \\
     &= \timeintegral \Eqtsmall\brs{g_t \modelsmall^2} dt - 2 \timeintegral\xintegral q_t \scoret{q_t} g_t \modelsmall  d\mb{x}dt + \timeintegral\Eqtsmall\brs{g_t\scoret{q_t}^2} dt \\
     &= \timeintegral \Eqtsmall\brs{g_t \modelsmall^2} dt - 2 
     \timeintegral\xintegral \partial_t q_t g_t \modelsmall  d\mb{x}dt + \timeintegral\Eqtsmall\brs{g_t\scoret{q_t}^2} dt, 
\end{align*}
where in the final line we have used $q_t \scoret{q_t} = q_t \partial_t \log q_t = \partial_t q_t$ to simplify. First note that the final term is a constant with respect to the model $\modelsmall$, and so we can write $C = \timeintegral\Eqtsmall\brs{g_t\scoret{q_t}^2} dt$. We continue by expanding the middle term via integration by parts
\begin{align}
\ourJ &= \timeintegral \Eqtsmall\brs{g_t \modelsmall^2} dt - 2 \brs{ \xintegral q_t g_t \modelsmall d\mb{x}}^{t=1}_{t=0} + 2 \timeintegral \xintegral q_t \partial_t (g_t \modelsmall) d\mb{x} dt + C \nonumber \\
      &= \timeintegral \Eqtsmall\brs{g_t \modelsmall^2} dt + 2 \timeintegral \xintegral q_t \partial_t (g_t \modelsmall) d\mb{x} dt + C \nonumber \\
      &= \timeintegral g_t \Eqtsmall\brs{\modelsmall^2} dt + 2 \timeintegral \partial_t g_t \Eqtsmall \brs{\modelsmall} dt + 2\timeintegral g_t \Eqtsmall\brs{\partial_t \modelsmall} dt + C \label{eq:app:deriv1},
\end{align}
where the second equality is due to $\brs{ \xintegral q_t g_t \modelsmall d\mb{x}}^{t=1}_{t=0} = 0$ as $g(0) = g(1) = 0$. 

% We continue off from the last line of \cref{app:SMderivation_1}, which is 
% \[
% \ourJ = \timeintegral g_t \Eqtsmall\brs{\modelsmall^2} dt + 2 \timeintegral \partial_t g_t \Eqtsmall \brs{\modelsmall} dt + 2\timeintegral g_t \Eqtsmall\brs{\partial_t \modelsmall} dt + C,
% \]
% as both derivations are the same until we specify a model $\modelsmall$. 
Let us now substitute the model given in \cref{eq:model}, stated again here for completeness, given by
\[
\modelsmall = \model = \brangle{\partialthetasmall, \mb{f}(\mb{x})} - \Eqtsmall \brs{\brangle{\partialthetasmall, \mb{f}(\mb{x})}}.
\]
We calculate $\Eqtsmall\brs{\modelsmall}$ and $\Eqtsmall\brs{\partial_t \modelsmall}$ to substitute into the equation above. These are given by
\begin{align*}
    \Eqtsmall\brs{\modelsmall} &= \Eqtsmall\brs{\brangle{\partialthetasmall, \mb{f}(\mb{x})} - \Eqtsmall \brs{\brangle{\partialthetasmall, \mb{f}(\mb{x})}}} \\
    &= \Eqtsmall\brs{\brangle{\partialthetasmall, \mb{f}(\mb{x})}} - \Eqtsmall \brs{\brangle{\partialthetasmall, \mb{f}(\mb{x})}} \\
    &= 0 \\
    \Eqtsmall\brs{\partial_t \modelsmall} &= \Eqtsmall\brs{\partial_t \br{\brangle{\partialthetasmall, \mb{f}(\mb{x})} - \Eqtsmall \brs{\brangle{\partialthetasmall, \mb{f}(\mb{x})}}}} \\
    &= \Eqtsmall\brs{\brangle{\partialdthetasmall, \mb{f}(\mb{x})} - \partial_t \br{\Eqtsmall \brs{\brangle{\partialthetasmall, \mb{f}(\mb{x})}}}} \\
    &= \Eqtsmall\brs{\brangle{\partialdthetasmall, \mb{f}(\mb{x})} - \partial_t \br{\xintegraltwo q_t \brangle{\partialthetasmall, \mb{f}(\mb{x})} d\mb{x}'}} \\
    &= \Eqtsmall\brs{\brangle{\partialdthetasmall, \mb{f}(\mb{x})} - \xintegraltwo\partial_t q_t \brangle{\partialthetasmall, \mb{f}(\mb{x})} d\mb{x}' - \xintegraltwo q_t \brangle{\partialdthetasmall, \mb{f}(\mb{x})} d\mb{x}' } \\
    &= \Eqtsmall\brs{\brangle{\partialdthetasmall, \mb{f}(\mb{x})} - \xintegraltwo\partial_t q_t \brangle{\partialthetasmall, \mb{f}(\mb{x})} d\mb{x}' - \Eqtsmall{ \brangle{\partialdthetasmall, \mb{f}(\mb{x})} d\mb{x}' } } \\ 
    &= \Eqtsmall\brs{\brangle{\partialdthetasmall, \mb{f}(\mb{x})} - \xintegraltwo\partial_t q_t \brangle{\partialthetasmall, \mb{f}(\mb{x})} d\mb{x}'} - \Eqtsmall \brs{ \brangle{\partialdthetasmall, \mb{f}(\mb{x})} d\mb{x}' } \\
    &= \Eqtsmall\brs{ - \xintegraltwo\partial_t q_t \brangle{\partialthetasmall, \mb{f}(\mb{x})} d\mb{x}' },
\end{align*}
where the integral $\xintegraltwo(\dots)d\mb{x}'$ is the same integral as $\xintegral(\dots)d\mb{x}$ but written as such to make them distinct from one another. Substituting these into \cref{eq:app:deriv1} gives
\begin{align*}
\ourJ &= \timeintegral g_t \Eqtsmall\brs{\modelsmall^2} dt - 2\timeintegral g_t \Eqtsmall\brs{ \xintegraltwo \partial_t q_t \brangle{\partialthetasmall, \mb{f}(\mb{x})} d\mb{x}' } dt + C \\
      &= \timeintegral g_t \Eqtsmall\brs{\modelsmall^2} dt - 2\timeintegral g_t \xintegral q_t \br{  \xintegraltwo \partial_t q_t \brangle{\partialthetasmall, \mb{f}(\mb{x})} d\mb{x}'}d\mb{x}  dt + C \\
      &\myeq{(a)} \timeintegral g_t \Eqtsmall\brs{\modelsmall^2} dt - 2\timeintegral g_t \br{\xintegral q_t d\mb{x}}  \xintegraltwo \partial_t q_t \brangle{\partialthetasmall, \mb{f}(\mb{x})} d\mb{x}' dt + C \\
      &\myeq{(b)} \timeintegral g_t \Eqtsmall\brs{\modelsmall^2} dt - 2\timeintegral g_t \xintegral \partial_t q_t \brangle{\partialthetasmall, \mb{f}(\mb{x})} d\mb{x} dt + C. 
\end{align*}
In the equality denoted by (a), we have used the fact that inside the integral $\xintegral q_t (\dots) d\mb{x}$ the only variable dependent on $\mb{x}$ was $q_t$, as $\mb{x}$ and $\mb{x}'$ are independent. We also have that $\xintegral q_t d\mb{x} = 1$ by $q_t$ being a probability density function. The equality denoted by (b) contains a re-labelling of $\mathcal{X} = \mathcal{X}'$ and $\mb{x} = \mb{x}'$, as they are the same variable, only labelled differently originally to make them distinct. We use integration by parts one final time to obtain
\begin{align*}
\ourJ &= \timeintegral g_t \Eqtsmall\brs{\modelsmall^2} dt - 2 \brs{\xintegral q_t g_t \brangle{\partialthetasmall, \mb{f}(\mb{x})} d\mb{x}}^{t=1}_{t=0} + 2 \timeintegral \xintegral q_t \partial_t \br{g_t \brangle{\partialthetasmall, \mb{f}(\mb{x})}} d\mb{x} dt + C \\
      &= \timeintegral g_t \Eqtsmall\brs{\modelsmall^2} dt + 2 \timeintegral \xintegral q_t \partial_t \br{g_t \brangle{\partialthetasmall, \mb{f}(\mb{x})}} d\mb{x} dt + C, 
\end{align*}
using again that $g(0) = g(1) = 0$, and finally
\begin{align*}
\ourJ &= \timeintegral g_t \Eqtsmall\brs{\modelsmall^2} dt + 2 \timeintegral \xintegral q_t \partial_t g_t \brangle{\partialthetasmall, \mb{f}(\mb{x})} d\mb{x} dt + 2\timeintegral\xintegral q_t g_t \brangle{\partialdthetasmall, \mb{f}(\mb{x})} d\mb{x} dt + C \\
      &= \timeintegral \Eqtsmall \brs{g_t \modelsmall^2 + 2 \partial_t g_t \brangle{\partialthetasmall, \mb{f}(\mb{x})} + 2 g_t \brangle{\partialdthetasmall, \mb{f}(\mb{x})}} dt
\end{align*}
which is the same as \cref{eq:deriv:objfinal} in the main text.
\section{Finite-sample Estimation Error of Lasso Estimator}
% In the following subsection, we focus on linear modeling where $\boldsymbol{\phi}(t) = t$ and paired data $\{(t_j, x_j)\}_{j=1}^n$, where $n$ denotes the total number of data points. 
{\color{red}don't need this definition in the main paper. Only need it in the appendix. }
%With these settings, let $X \in \mathbb{R}^{n \times k}$, where the $l$-th row of $X$ is $\boldsymbol{f}(x_{l})^\top$, and $\boldsymbol{\alpha}r{X} \in \mathbb{R}^{n \times k}$, where $i$-th row of $\boldsymbol{\alpha}r{X}$ is $\mathbb{E}_{q_{t_{i}}}[\boldsymbol{f}(x)]^\top$. 

%Defining $X^o = X - \boldsymbol{\alpha}r{X}$, 
An equivalent sample objective function is as the following:
\begin{equation}
     \hat{J}(\boldsymbol{\alpha}) =  \frac{1}{2n}\left[\boldsymbol{\alpha} {X^o}^\top \boldsymbol{G}X^o  \boldsymbol{\alpha}^\top+
    2\boldsymbol{1}_n^\top \partial_t \boldsymbol{G}X\boldsymbol{\alpha}^\top \right]\label{lafeq} 
\end{equation}
where diagonal matrix $\boldsymbol{G},\partial_t \boldsymbol{G}\in \mathbb{R}^{n\times n}$ with $i$-th diagonal entry to be  $g(t_{i})$ and $\partial_t g(t_i)$ respectively.
\subsection{Proof of Theorem \ref{consi}}\label{consistency}
Following equation \ref{lafeq} and Assumption \ref{ass:alphastar}, we can express the second order Taylor polynomial around $\boldsymbol{\alpha}^\star$ as follows:
\begin{equation}
    \hat{J}(\hat{\boldsymbol{\alpha}}) = \hat{J}(\boldsymbol{\alpha}^\star) + \frac{1}{n} \left[ 
\boldsymbol{\alpha}^\star{X^o}^\top \boldsymbol{G}{X^o}\boldsymbol  +  \boldsymbol{1}_n^\top \partial_t \boldsymbol{G} X\right](\boldsymbol{\hat{\alpha}} - \boldsymbol{\alpha}^\star)^\top+ \frac{1}{2n}(\boldsymbol{\hat{\alpha}} - \boldsymbol{\alpha}^\star) \left[ 
{X^o}^\top \boldsymbol{G}{X^o}\right](\hat{\boldsymbol{\alpha}} - \boldsymbol{\alpha}^\star)^\top
\end{equation}
where the residual $R_2(\hat{\boldsymbol{\alpha}}, \boldsymbol{\alpha}^\star) = 0$ since $\hat{J}$ quadratic.

\begin{theorem}
    Under condition $\lambda_{\boldsymbol{\alpha}} \geq 2 \left\|\nabla_{\boldsymbol{\alpha}} \hat{J}(\boldsymbol{\alpha}^\star)\right\|_\infty$, the error vector $\widehat{\Delta} = \hat{\boldsymbol{\alpha}}- \boldsymbol{\alpha}^\star \in \mathbb{C}_{3}(S)$
\end{theorem}
\begin{proof}
Since $\hat{\boldsymbol{\alpha}}$ is optimal, we have 
\begin{equation}
        \hat{J}(\hat{\boldsymbol{\alpha}}) + \lambda_{\boldsymbol{\alpha}} ||\hat{\boldsymbol{\alpha}}||_1 \leq \hat{J}(\boldsymbol{\alpha}^\star) + \lambda_{\boldsymbol{\alpha}} ||{\boldsymbol{\alpha}}^\star||_1
\end{equation}
{\color{red} bold font for matrices}
Rearranging we have from second order Taylor approximation:
\begin{equation}
    0 \leq \frac{1}{2n}||G^{\frac{1}{2}}{X^o}\hat{\Delta}^\top||_2^2 \leq \frac{1}{n} |\nabla_{\boldsymbol{\alpha}}\hat{J}(\boldsymbol{\alpha}^\star)\hat{\Delta}^\top| + \lambda_{n}\{||\boldsymbol{\alpha}^\star||_1 - ||\hat{\boldsymbol{\alpha}}||_1\}
\end{equation}
where $|\cdot|$ denote the absolute value. Now since $\boldsymbol{\alpha}^\star$ is $S$-sparse, we can write 
\begin{equation}
\|\boldsymbol{\alpha}^\star\|_1-\|\hat{\boldsymbol{\alpha}}\|_1=\|\boldsymbol{\alpha}_S^\star\|_1-\|\boldsymbol{\alpha}_S^\star+\widehat{\Delta}_S\|_1-\|\widehat{\Delta}_{S^c}\|_1.
\end{equation}
Using Holder’s inequality and the triangle inequality, we have
\begin{align}
    0 &\leq \frac{1}{n}||G^{\frac{1}{2}}{X^o}\hat{\Delta}^\top||_2^2 \leq 2|\nabla_{\boldsymbol{\alpha}}\hat{J}(\boldsymbol{\alpha}^\star)\hat{\Delta}^\top| + 2\lambda_{\boldsymbol{\alpha}} \{ \|\boldsymbol{\alpha}_S^\star\|_1 - \|\boldsymbol{\alpha}^\star_S+\widehat{\Delta}_S\|_1 - \|\widehat{\Delta}_{S^c}\|_1 \} \\
    &\leq  2\|\nabla_{\boldsymbol{\alpha}}\hat{J}(\boldsymbol{\alpha}^\star)\|_\infty \|\widehat{\Delta}\|_1 + 2\lambda_{\boldsymbol{\alpha}} \{ \|\widehat{\Delta}_S\|_1 - \|\widehat{\Delta}_{S^c}\|_1 \} \\
    &\leq \lambda_{\boldsymbol{\alpha}} \{ 3\|\widehat{\Delta}_S\|_1 - \|\widehat{\Delta}_{S^c}\|_1 \},
\end{align}
where last inequality shows that $\widehat{\Delta} \in \mathbb{C}_{3}(S)$.
\end{proof}
\begin{theorem}
 $||\widehat{\Delta}||_1 \leq 2 \sqrt{s}||\widehat{\Delta}||_2$ where $s = |S|$.\end{theorem}
 \begin{proof}
Since $S$ is the support of $\alpha^\star$
\begin{align}
    &||\boldsymbol{\alpha}_S^\star||_1 = ||\boldsymbol{\alpha}^\star||_1 \geq ||\boldsymbol{\alpha}^\star + \widehat{\Delta}||_1 
    = ||\boldsymbol{\alpha}_S^\star + \widehat{\Delta}_S||_1 + ||\widehat{\Delta}_{S^c}||_1 
    \geq ||\boldsymbol{\alpha}^\star_S||_1 - ||\widehat{\Delta}_S||_1 + ||\widehat{\Delta}_{S^c}||_1.
\end{align}
where we used the fact that $\boldsymbol{\alpha}_{S^c}^\star = 0 $ and triangle inequality. This implies that $\widehat{\Delta} \in \mathbb{C}_1(S)$. Therefore
\begin{equation}
    ||\widehat{\Delta}||_1 = ||\widehat{\Delta}_S||_1 + ||\widehat{\Delta}_{S^c}||_1 \leq 2 ||\widehat{\Delta}_S||_1  \leq 2\sqrt{s} ||\widehat{\Delta}||_2
\end{equation}
\end{proof}
With all above, we can then apply the RE condition.  Finally we have $||\widehat{\Delta}||_2^2 \leq \frac{3}{\kappa}\lambda_{\boldsymbol{\alpha}} \sqrt{s} ||\widehat{\Delta}||_2$, which implies that 
\begin{equation}
    ||\hat{\boldsymbol{\alpha}} - \boldsymbol{\alpha}^\star||_2 \leq \frac{3}{\kappa}\lambda_{\boldsymbol{\alpha}} \sqrt{s}
\end{equation}

\subsection{Proof of Theorem \ref{probineqconst}}\label{pf:probineqconst}

We have $\nabla_{\boldsymbol{\alpha}}\hat{J}(\boldsymbol{\alpha}) = \frac{1}{n} \sum_{j=1}^{n} \nabla_{\boldsymbol{\alpha}}\boldsymbol{m_{\alpha}}(t_j,\boldsymbol{x}_j)
$. %Recall that $\nabla_{\boldsymbol{\alpha}}\boldsymbol{m_\alpha}(t,\boldsymbol{x}) = \boldsymbol{{\alpha}}\left(\boldsymbol{f(x)} - \mathbb{E}_{q_{t}}[\boldsymbol{f(x)}]\right) g(t) \left(\boldsymbol{f(x)} - \mathbb{E}_{q_t}[\boldsymbol{f(x)}]\right) + (\partial_t g(t)) \boldsymbol{f(x)}.$
Therefore, the covariance matrix of $\nabla_{\boldsymbol{\alpha}}\boldsymbol{m_\alpha}(t,\boldsymbol{x})$ is a constant matrix which can be estimated by estimating the variance of $\mathbb{E}_{q_t}(\boldsymbol{f(x)})$ and $\partial_t g(t)$, when the variance of $\boldsymbol{f(x)}$ is known. 

\begin{lemma}
    Under the condition that the r.v. $\boldsymbol{f}(x) $ is bounded, let $\sigma^2 = \max_{1\leq i\leq k} \boldsymbol{\Sigma}_{ii}$, where $\boldsymbol{\Sigma}$ is the covariance matrix of the random variable $\nabla_{\boldsymbol{\alpha}} \boldsymbol{m_{\alpha}}(t,\boldsymbol{x}) \big|_{\boldsymbol{\alpha}=\boldsymbol{\alpha}^\star}$, the elements of $\nabla_{\boldsymbol{\alpha}} \hat{J} (\boldsymbol{\alpha}) \big|_{\boldsymbol{\alpha} = \boldsymbol{\alpha}^\star}$ follow a zero-mean sub-Gaussian distribution with parameter $\sigma^2/n$.
\end{lemma}
\begin{proof}
\textbf{(1) Proof the sub-Gaussian: }
let $|g_t|\leq C_g \in \mathbb{R}_{+}, |\partial_tg_t|\leq C_{\partial_t g_t} \in \mathbb{R}_{+}, ||\mathbb{E}_{q_t}[\boldsymbol{f}(x)]||\leq C_{E} \in \mathbb{R}_{+}$ and $||\boldsymbol{f}(x)|| \leq C_f \in \mathbb{R}_{+}$ for $t \in [0,1]$, where $||\cdot||$ denotes some vector norm. By using triangle inequality in $(i),(iii)$ and Cauchy-Schwarz inequality in $(ii)$ , we have 

\begin{align}
   \left\| \nabla_{\boldsymbol{\alpha}} \hat{J} \left( \boldsymbol{\alpha} \right) \bigg|_{\boldsymbol{\alpha} = \boldsymbol{\alpha}^\star} \right\|
    &\stackrel{(i)}{\leq} \frac{1}{n} \left\| \boldsymbol{\alpha}^\star X^{o \top} G X^o \right\| + \frac{1}{n} \left\| \boldsymbol{1}_n \tilde{G} X \right\| \nonumber \\
    & \leq C_g \left\| \frac{1}{n} \boldsymbol{\alpha}^\star X^{o \top} X^o \right\| + C_{\partial_t g_t} \left\| \frac{1}{n} \boldsymbol{1}_n X \right\| \nonumber \\
    &\stackrel{(ii)}{\leq} C_g \left\| \boldsymbol{\alpha}^\star \right\| \cdot \left\| \frac{1}{n} X^{o \top} X^o \right\| + C_{\partial_t g_t} \left\| \frac{1}{n} \sum^{n}_{i=1} \boldsymbol{f}(x_i) \right\| \nonumber \\
    &\stackrel{(iii)}{\leq} C_g \left\| \boldsymbol{\alpha}^\star \right\| \cdot \left( \frac{1}{n} \sum^{n}_{i=1} \left( \left\| \boldsymbol{f}(x_i) \right\| + \left\| \mathbb{E}_{q_{t_{i}}}[\boldsymbol{f}(x)] \right\| \right) \right)^2 + C_{\partial_t g_t} \frac{1}{n} \sum^{n}_{i=1} \left\| f(x) \right\| \nonumber \\
    & \leq \left\| \boldsymbol{\alpha}^\star \right\| \left( C_g (C_f + C_E)^2 + C_f C_{\partial_t g_t} \right) \in \mathbb{R}
\end{align}

Let $M = ||\boldsymbol{\alpha}^\star||(C_g(C_f+C_E)^2 + CC_{\partial_t g_t})$ for simplicity. A general property of norms is that they dominate the maximum absolute value of the vector components, that is,
 \[
  \left\|\nabla_{\boldsymbol{\alpha}} \hat{J}(\boldsymbol{\alpha}) \bigg|_{\boldsymbol{\alpha}=\boldsymbol{\alpha}^\star}\right\| \geq \max_{1\geq i \geq k}|J_i| \geq |J_l| \text{ for all } 1\leq l \leq k 
 \]
where $J_j$ denotes $j$-th element of  $\nabla_{\boldsymbol{\alpha}}\hat{J}(\boldsymbol{\alpha}^\star)$. Thus we have $|J_l| \leq M \text{ for all } 1\leq l \leq k$, which implies that  $\nabla_{\boldsymbol{\alpha}}\hat{J}(\boldsymbol{\alpha}^\star)$ is element-wise bounded hence all elements are sub-Gaussian by \cite{hoeffding1994probability}. 
Therefore, fixed number of data points $n$, then each element of $\nabla_{\boldsymbol{\alpha}}\hat{J}(\boldsymbol{\alpha}^\star)$ follows a sub-Gaussian distribution with parameter $\sigma^2/n$ by addition rule of variance.
\\
\textbf{(2) Proof of zero-mean: }We also assert that $\nabla_{\boldsymbol{\alpha}}\hat{J}(\boldsymbol{\alpha}^\star) \in \mathbb{R}^k$ is a zero-mean random variable. Recall that the conditional density function $q(x|t)$ as $q_t(x)$ where $q_t:\mathbb{R}^k\rightarrow \mathbb{R}$ and $q: \mathbb{R}\rightarrow\mathbb{R}$ represent the density of $t$, where $t$ is uniformly distributed in the domain $[0,1]$, we then have the following:
\begin{align}
    &\mathbb{E}_{x\sim q_t(x),\,t\sim q(t)}\left[\nabla_{\boldsymbol{\alpha}}\hat{J}(\boldsymbol{\alpha})\big|_{\boldsymbol{\alpha}=\boldsymbol{\alpha}^\star}\right] \notag &\\
    &= \frac{1}{n}\mathbb{E}_{x\sim q_t(x),\, t\sim q(t)}\left[\boldsymbol{\alpha}^\star{(X-{X}^o)}^\top \boldsymbol{G}{(X-{X}^o)} + \boldsymbol{1}_n^\top \partial_t \boldsymbol{G} X\right] \label{eq:1} &\\
    &\stackrel{(i)}{=} \mathbb{E}_{x\sim q_t(x),\, t\sim q(t)}\left[\boldsymbol{{\alpha}^\star}{\left(\boldsymbol{f}(x)-\mathbb{E}_{q_t}[\boldsymbol{f}(x)]\right)} g_t{\left(\boldsymbol{f}(x)-\mathbb{E}_{q_t}[\boldsymbol{f}(x)]\right)} + (\partial_t g_t) \boldsymbol{f}(x)\right] \label{eq:2} &\\
    &= \int_t \int_x q(t) q_t(x)\{
    \boldsymbol{{\alpha}^\star}{(\boldsymbol{f}(x)-\mathbb{E}_{q_t}[\boldsymbol{f}(x)])}g_t\left(\boldsymbol{f}(x)-\mathbb{E}_{q_t}[\boldsymbol{f}(x)]\right)
    + (\partial_t g_t) \boldsymbol{f}(x)
    \} \mathrm{d}x \, \mathrm{d}t\\
    &\stackrel{(ii)}{=} \int_t \int_x q_t(x)\{
    (\partial_t\log q_t(x)) g_t\left(\boldsymbol{f}(x)-\mathbb{E}_{q_t}[\boldsymbol{f}(x)]\right)
    + (\partial_t g_t) \boldsymbol{f}(x)
    \} \mathrm{d}x \, \mathrm{d}t\\
    &= \int_t \int_x 
    (\partial_t q_t(x)) g_t \left(\boldsymbol{f}(x)-\mathbb{E}_{q_t}[\boldsymbol{f}(x)]\right)
    + q_t(x) (\partial_t g_t) \boldsymbol{f}(x)
    \} \mathrm{d}x \, \mathrm{d}t\\
    &= [q_t(x) g_t\left(\boldsymbol{f}(x)-\mathbb{E}_{q_t}[\boldsymbol{f}(x)]\right)]^{t=1}_{t=0} 
    -\int_t \int_x q_t(x)
    \partial_t \left[ g_t \left( \boldsymbol{f}(x)-\mathbb{E}_{q_t}[\boldsymbol{f}(x)]\right)\right]
    - q_t(x) (\partial_t g_t)\boldsymbol{f}(x) \mathrm{d}x \, \mathrm{d}t\\
    &\stackrel{(iii)}{=} \int_t \int_x -q_t(x)
    \left[ (\partial_t g_t) \left(\boldsymbol{f}(x)-\mathbb{E}_{q_t}[\boldsymbol{f}(x)]\right) + g_t \partial_t \mathbb{E}_{q_t}\left[ \boldsymbol{f}(x)\right] \right]
    + q_t(x)  (\partial_t g_t)\boldsymbol{f}(x) \mathrm{d}x \, \mathrm{d}t\\ 
    &= \int_t \int_x q_t(x)
    \left( [\partial_t g_t]  \mathbb{E}_{q_t}[\boldsymbol{f}(x)] + g_t \partial_t \mathbb{E}_{q_t}[\boldsymbol{f}(x)] \right)
     \mathrm{d}x \, \mathrm{d}t = \int_t \int_x q_t(x) \partial_t [g_t \mathbb{E}_{q_t}[\boldsymbol{f}(x)]] \mathrm{d}x \, \mathrm{d}t\\
    &= [q_t(x)g_t\mathbb{E}_{q_t}[\boldsymbol{f}(x)]]^{t=1}_{t=0} -\int_t \int_x (\partial_t q_t(x)) g_t \mathbb{E}_{q_t}[\boldsymbol{f}(x)] \mathrm{d}x \, \mathrm{d}t\\     
    &\stackrel{(iv)}{=} -\int_t \partial_t \left(\int_x  q_t(x) \mathrm{d}x \,\right) g_t \mathbb{E}_{q_t}[\boldsymbol{f}(x)]  \mathrm{d}t = \boldsymbol{0}
\end{align}
where $(i)$ follows that $\{f(x_1),..,f(x_n)\}$ are i.i.d; $(ii)$ follows from the definition of $\partial_t \log q_t(x)$ and $q(t) = 1$; $(iii),(iv)$ uses the boundary condition of $g(t)$. Therefore, each element of $\nabla_{\boldsymbol{\alpha}}\hat{J}(\boldsymbol{\alpha}^\star)$ is a zero-mean sub-Gaussian r.v. 

\end{proof}
\begin{lemma}\label{lemma:Jexp}
Let $J_i$ denotes i-th element of  $\nabla_{\boldsymbol{\alpha}}\hat{J}(\boldsymbol{\alpha}^\star)$, we have 
\begin{equation}
    \mathbb{E}[\max_{i\in [k]} |J_i|] \leq  \sqrt{\frac{2\sigma^2 \log k}{n}}
\end{equation}
\end{lemma}
\begin{proof}
 We have \(\{J_i\}_{i=1}^k\) is a sequence of zero-mean random variables, each follows sub-Gaussian with parameter \(\sigma^2 /n\). For any \(\lambda > 0\), we can use the convexity of the exponential function to obtain
\[
\exp\{\lambda \mathbb{E}[\max_{i \in [k]} J_i]\} \leq \mathbb{E}[\exp\{\lambda \max_{i \in [k]} J_i\}]
\]
by Jensen's inequality. And by the monotonicity of the exponential
\[
\mathbb{E}[\exp\{\lambda \max_{i \in [k]} J_i\}] = \mathbb{E}[\max_{i \in [k]} e^{\lambda J_i}] \leq \sum_{i=1}^{k} \mathbb{E}[e^{\lambda J_i}] \leq k e^{\frac{\lambda^2 \sigma^2}{2n}}.
\]
where last inequality follows the definition of sub-Gaussian r.v. Therefore,
\[
\mathbb{E}[\max_{i \in [k]} J_i] \leq \frac{\log k}{\lambda} + \lambda \frac{\sigma^2}{2n}
\]
and \(\lambda = \sqrt{\frac{2n \log k}{\sigma^2}}\) is optimal in $\lambda>0$; substituting we have 
\begin{equation}
\mathbb{E}\left[\max_{i \in [k]} J_i\right] \leq \frac{\sigma}{\sqrt{2n}} \sqrt{\log k} + \frac{\sigma}{\sqrt{2n}} \sqrt{\log k} = \sqrt{2 \sigma^2 \log k/n} \label{expconst}
\end{equation}
Since \ref{expconst} does not assume independence between individual \(J_i\). The result follows by
\[
    \max_{i \in [k]} |J_i| = \max \{|J_1|, \ldots, |J_k|\} = \max \{J_1, \ldots, J_n, -J_1, \ldots, -J_k\}
\]
\end{proof}
Consequently, from standard sub-Gaussian tail bound and definition of $l_{\infty}$ norm, we have
\begin{equation}
    \mathbb{P}\left[ \left\|\nabla_{\boldsymbol{\alpha}} \hat{J}(\boldsymbol{\alpha}) \bigg|_{\boldsymbol{\alpha}=\boldsymbol{\alpha}^\star}\right\|_{\infty} \geq \sigma\left(\sqrt{\frac{2\log k}{n}}+\delta \right) \right]\leq 2e^{-\frac{n\delta^2}{2}} \;\; \text{for all } \delta>0
\end{equation}
Hence if we set $\lambda_{\boldsymbol{\alpha}}  = 2\sigma\left(\sqrt{\frac{2\log k}{n}}+\delta\right)$, then we have the probability that $\lambda_{\boldsymbol{\alpha}} \geq 2||\nabla_{\boldsymbol{\alpha}}\hat{J}(\boldsymbol{\alpha}^\star)||_{\infty}$ is in rate $1-2\exp\{-\Theta(n\delta^2)\}$, which implies 
\begin{equation}
    ||\hat{\boldsymbol{\alpha}} - \boldsymbol{\alpha}^\star||_2 \leq \frac{6}{\kappa}\sqrt{s}\sigma\left(\sqrt{\frac{2\log k}{n}}+\delta\right)
\end{equation}
with probability greater than $1-2\exp\{-\frac{n\delta^2}{2}\}$ for all $\delta>0$.

\section{Asymptotic Distribution Derivation under the No Change Hypothesis} \label{app:asymptotic}

Following \cref{sec:estimating:partialtheta} and \cref{ass:alphastar}, we have
\[
\partialthetasmall = \modeldtheta,
\]
where $\mb\alpha \in \R^{b \times k}$ and $\partial_t \mb\phi(t) \in \R^b$. Note that $b$ refers to the dimension of the features given by $\mb\phi(t)$ which changes depending on the model for $\mb\phi(t)$. 

\subsection{A Note on Matrix Sizes and Reshaping}

Since $\mb\alpha$ is a $(b \times k)$-matrix, to derive its asymptotic distribution, we reshape $\mb\alpha$ to a separate vector $\widetilde{\mb{\alpha}} \in \R^{bk}$ without loss of generality. Further, we also define separate vectors $\partial_t \widetilde{\mb\phi}(t) \in \R^{bk \times k}$ and $\partial_t^2 \widetilde{\mb\phi}(t) \in \R^{bk \times k}$, defined such that $\modeldthetatilde = \modeldtheta$ and $\modelddthetatilde = \modelddtheta$. All these new variables are defined as follows:
\[
\partial_t \widetilde{\mb\phi}(t) = \begin{bmatrix}
    \partial_t \mb\phi(t) & \mb{0}_b &  \dots  & \mb{0}_b \\
    \mb{0}_b & \partial_t \mb\phi(t) &  \dots  & \mb{0}_b \\
    \vdots   & \vdots               &  \ddots & \vdots \\
    \mb{0}_b & \mb{0}_b             &  \dots  & \partial_t \mb\phi(t)
\end{bmatrix}, \qquad
\partial_t^2 \widetilde{\mb\phi}(t) = \begin{bmatrix}
    \partial_t^2 \mb\phi(t) & \mb{0}_b &  \dots  & \mb{0}_b \\
    \mb{0}_b & \partial_t^2 \mb\phi(t) &  \dots  & \mb{0}_b \\
    \vdots   & \vdots               &  \ddots & \vdots \\
    \mb{0}_b & \mb{0}_b             &  \dots  & \partial_t^2 \mb\phi(t)
\end{bmatrix}, \qquad
\widetilde{\mb\alpha} = \begin{bmatrix}
    \alpha_{1, 1} \\ \vdots \\ \alpha_{b, 1} \\ \alpha_{1, 2} \\ \vdots \\ \alpha_{b, k}
\end{bmatrix}
\]
The reason and motivation for this reshaping should hopefully become clear by the end of this section. In summary, it is so we can derive the asymptotic distribution for $\widetilde{\mb\alpha}$ as a vector, and the results will carry forward to $\mb\alpha$.

For convenience and brevity, for the remainder of this section we will \textit{not} rename instances of $\mb\alpha$ as $\widetilde{\mb\alpha}$, nor $\partial_t \widetilde{\mb\phi}(t)$ or $\partial_t \widetilde{\mb\phi}(t)$, and they will remain as their original, non-tilde variants.

\subsection{\texorpdfstring{Asymptotic Distribution of $\sqrt{n}(\widehat{\mb{\alpha}} - \mb{\alpha}^\star)$}{Asymptotic Distribution of sqrt(n)(alpha_hat - alpha_star)}}

Recall our sample objective function, given by 
\begin{equation}
\ourJhat = \frac{1}{T} \sum^T_{j=1} \frac{1}{{n}} \sum^{n}_{i=1} m_{\mb\alpha}(\mb{x}_i, t_j) = \frac{1}{T} \sum^T_{j=1} m_n(\mb{\alpha}, t_j),
\label{eq:app:sampleobj}
\end{equation}
where for convenience of notation we have written $m_n(\mb{\alpha}, t) = \frac{1}{{n}} \sum^{n}_{i=1} m_{\mb\alpha}(\mb{x}_i, t)$, and  
\begin{align}
m_{\mb{\alpha}}(\mb{x}, t) &= g(t) \modelsmallsample{t}^2 + 2   \partial_t g(t)\brangle{\partialtheta,\mb{f}(\mb{x})} + 2g(t)\brangle{\partialdtheta,\mb{f}(\mb{x})} \nonumber \\
   &= g(t) \brangle{\modeldtheta, \mb{f} - \Eqtsmall\brs{\mb{f}}}^2 + 2 \brangle{\partial_t g(t)\modeldtheta + g(t)\modelddtheta, \mb{f}}, \label{eq:app:m}
\end{align}
where we have abbreviated $\mb{f} = \mb{f}(\mb{x})$, and the dependence on $\mb{x}$ is implied. 

Denote by 
\begin{align*}
\mb{m}_n'(\mb{\alpha}_0, t) &= \frac{1}{{n}} \sum^{n}_{i=1} \mb\nabla_{\mb\alpha} m_{\mb\alpha}(\mb{x}_i, t)\big\vert_{\mb\alpha = \mb\alpha_0}, \\
\mb{m}_n''(\mb{\alpha}_0, t) &= \frac{1}{{n}} \sum^{n}_{i=1} \mb\nabla_{\mb\alpha}^2 m_{\mb\alpha}(\mb{x}_i, t)\big\vert_{\mb\alpha = \mb\alpha_0}, \\
\mb{m}_n'''(\mb{\alpha}_0, t) &= \frac{1}{{n}} \sum^{n}_{i=1} \mb\nabla_{\mb\alpha}^3 m_{\mb\alpha}(\mb{x}_i, t)\big\vert_{\mb\alpha = \mb\alpha_0},
\end{align*}
the first, second and third derivative, respectively, of $m_n(\mb{\alpha}, t)$ with respect to $\mb\alpha$, evaluated at $\mb\alpha_0$. Let $\widehat{\mb\alpha}$ be the minimiser of the sample objective, given by \cref{eq:app:sampleobj}, therefore
\begin{equation}
    \frac{1}{T}\sum^T_{j=1}\mb{m}_n'(\widehat{\mb{\alpha}}, t_j) = \mb{0}, \label{eq:app:alphahatcon}
\end{equation}
\cref{ass:alphastar} states that $\mb\alpha^\star$ is the true parameter value under the model $\partialthetastarsmall = {\mb\alpha^\star}^\top (\partial_t \mb\phi(t))$, such that
\begin{equation}
\timeintegral \E \brs{\mb\nabla_{\mb\alpha} m_{\mb\alpha}(\mb{x}, t)\big\vert_{\mb\alpha = \mb\alpha^\star}}dt = \mb{0}. \label{eq:app:alphastarcon}
\end{equation}
Now consider the Taylor expansion of $\mb{m}_n'(\widehat{\mb{\alpha}}, t)$ around $\mb\alpha^\star$, given by
\begin{align*}
\mb{m}_n'(\hat{\mb{\alpha}}, t) &= \mb{m}_n'(\mb\alpha^\star, t) + (\hat{\mb\alpha} - \mb\alpha^\star) \mb{m}_n''(\mb\alpha^\star, t) + \frac{1}{2}(\hat{\mb\alpha} - \mb\alpha^\star)^2 \mb{m}_n'''(\mb\alpha^\star, t) \\
  & = \mb{m}_n'(\mb\alpha^\star, t) + (\hat{\mb\alpha} - \mb\alpha^\star) \mb{m}_n''(\mb\alpha^\star, t),
\end{align*}
where we have used that $\mb{m}_n'''(\mb{\alpha}, t) = 0$ due to $m_{\mb{\alpha}}(\mb{x}, t)$ being a quadratic function with respect to $\mb\alpha$. From the above, we can apply the sum on both sides to write
\[
\frac{1}{T} \sum_{j=1}^T  \mb{m}_n'(\hat{\mb{\alpha}}, t) = \frac{1}{T} \sum_{j=1}^T \mb{m}_n'(\mb\alpha^\star, t_j) + (\hat{\mb\alpha} - \mb\alpha^\star) \frac{1}{T} \sum_{j=1}^T\mb{m}_n''(\mb\alpha^\star, t_j)  = 0,
\]
where the final equality comes from \cref{eq:app:alphahatcon}. We can rearrange and then multiply by $\sqrt{n}$ on both sides to give
\begin{equation}
\sqrt{n}(\widehat{\mb\alpha} - \mb\alpha^\star) = \underbrace{\br{\frac{1}{T}\sum_{j=1}^T\mb{m}_n''(\mb\alpha^\star, t_j) }}_{(a)}{\vphantom{\sum^N_i}}^{-1} \underbrace{\br{\frac{1}{T}\sum_{j=1}^T \sqrt{n} \mb{m}_n'(\mb\alpha^\star, t_j)}}_{(b)}.
\label{eq:app:alphaminusalphastar}
\end{equation}
We can study the right hand side of \cref{eq:app:alphaminusalphastar} to understand its asymptotic distribution and therefore find an asymptotic distribution for $\sqrt{n}(\widehat{\mb\alpha} - \mb\alpha^\star)$. In order, we will consider the asymptotic properties of both (a) and (b) as $n \to \infty$ and $T \to \infty$.

% first term
\paragraph{(a)} 

By the law of large numbers, 
\begin{equation}
\mb{m}_n''(\mb\alpha^\star, t) = \frac{1}{n} \sum^{n}_{i=1} \mb\nabla_{\mb\alpha}^2 m_{\mb\alpha}(\mb{x}_i, t)\big\vert_{\mb\alpha = \mb\alpha^\star} \;\xrightarrow{\; P \;}\; \Eqtsmall \brs{ \mb\nabla_{\mb\alpha}^2 m_{\mb\alpha}(\mb{x}, t)\big\vert_{\mb\alpha = \mb\alpha^\star}}
\label{eq:app:asymptotic_terma1}
\end{equation}
and therefore 
\[
\frac{1}{T}\sum^T_{j=1} \mb{m}_n''(\mb\alpha^\star, t_j)   \xrightarrow{\; P \;} \frac{1}{T}\sum^T_{j=1}\Eqtsmall\brs{\mb\nabla_{\mb\alpha}^2 \mb{m}_{\mb\alpha}(\mb{x}, t_j)\big\vert_{\mb\alpha = \mb\alpha^\star}},
\]
because the dependence on $t$ in \cref{eq:app:asymptotic_terma1} is not related to the convergence in probability.

\paragraph{(b)}

By the central limit theorem, when $n \to \infty$,
\begin{align*}
\sqrt{n} \; \mb{m}_n'(\mb\alpha^\star, t) = \frac{1}{\sqrt{n}} \sum^{n}_{i=1} \mb\nabla_{\mb\alpha} m_{\mb\alpha}(\mb{x}_i, t)\big\vert_{\mb\alpha = \mb\alpha^\star} \xrightarrow{\; d \;}\;  \mathcal{N}\br{\E \brs{\mb\nabla_{\mb\alpha} m_{\mb\alpha}(\mb{x}_i, t)\big\vert_{\mb\alpha = \mb\alpha^\star}} , \operatorname{Var}\brs{\mb\nabla_{\mb\alpha} m_{\mb\alpha}(\mb{x}_i, t)\big\vert_{\mb\alpha = \mb\alpha^\star}}} 
\end{align*}
and hence
\[
\frac{1}{T}\sum^T_{j=1}\sqrt{n}\hspace{0.25mm}\mb{m}_n'(\mb\alpha^\star, t_j) \xrightarrow{\; d \;} \mathcal{N} \br{\frac{1}{T} \sum^T_{j=1} \E \brs{\mb\nabla_{\mb\alpha} m_{\mb\alpha}(\mb{x}_i, t_j)\big\vert_{\mb\alpha = \mb\alpha^\star}} , \frac{1}{T^2}\sum^T_{j=1}\mathrm{Var}[\mb\nabla_{\mb\alpha} m_{\mb\alpha}(\mb{x}_i, t_j)\big\vert_{\mb\alpha = \mb\alpha^\star}]}.
\]
Since we are studying in the case of $T \to \infty$, we can also write
\[
\frac{1}{T} \sum^T_{j=1} \E \brs{\mb\nabla_{\mb\alpha} m_{\mb\alpha}(\mb{x}_i, t_j)\big\vert_{\mb\alpha = \mb\alpha^\star}} \xrightarrow{\; P \;} \timeintegral \E \brs{\mb\nabla_{\mb\alpha} m_{\mb\alpha}(\mb{x}_i, t)\big\vert_{\mb\alpha = \mb\alpha^\star}}dt = \mb{0}
\]
by definition of $\mb\alpha^\star$ as given in \cref{eq:app:alphastarcon}. Therefore we can say, overall,
\begin{equation}
    \frac{1}{T}\sum^T_{j=1}\mb{m}'_n(\mb\alpha^\star, t_j) \xrightarrow{\; d \;} \mathcal{N} \br{\mb{0}, \frac{1}{T^2}\sum^T_{j=1}\mathrm{Var}[\mb\nabla_{\mb\alpha} m_{\mb\alpha}(\mb{x}_i, t_j)\big\vert_{\mb\alpha = \mb\alpha^\star}]}.
\end{equation}

% \paragraph{Combining (a) and (b)}

To combine both (a) and (b) together to determine the convergence in distribution of $\sqrt{n}(\widehat{\mb\alpha} - \mb\alpha^\star)$, we use Slutsky's Theorem. Since (b) converges in probability and (a) converges in distribution, the product of the two converges in distribution which is given by
\[
\sqrt{n}(\widehat{\mb\alpha} - \mb\alpha^\star) = \br{\frac{1}{T}\sum_{j=1}^T\mb{m}_n''(\mb\alpha^\star, t_j) }{\vphantom{\sum^N_i}}^{-1} \br{\frac{1}{T}\sum_{j=1}^T \sqrt{n} \mb{m}_n'(\mb\alpha^\star, t_j)} \xrightarrow{\; d \;} \mathcal{N}\br{\mb{0}, \mb{\Sigma}_{\mb\alpha}},
\]
where
\begin{align}
\mb\Sigma_{\mb\alpha} &= \br{\frac{1}{T}\sum^T_{j=1}\E\brs{\mb\nabla_{\mb\alpha}^2 \mb{m}_{\mb\alpha}(\mb{x}, t_j)\big\vert_{\mb\alpha = \mb\alpha^\star}}}^{-1} \frac{1}{T^2}\sum^T_{j=1} \mathrm{Var}\brs{\mb\nabla_{\mb\alpha} \mb{m}_{\mb\alpha}(\mb{x}, t_j)\big\vert_{\mb\alpha = \mb\alpha^\star}} \br{\frac{1}{T}\sum^T_{j=1}\E\brs{\mb\nabla_{\mb\alpha}^2 \mb{m}_{\mb\alpha}(\mb{x}, t_j)\big\vert_{\mb\alpha = \mb\alpha^\star}}}^{-1} \nonumber \\
 &= \br{\sum^T_{j=1}\E\brs{\mb\nabla_{\mb\alpha}^2 \mb{m}_{\mb\alpha}(\mb{x}, t_j)\big\vert_{\mb\alpha = \mb\alpha^\star}}}^{-1} \sum^T_{j=1} 
 \mathrm{Var}\brs{\mb\nabla_{\mb\alpha} \mb{m}_{\mb\alpha}(\mb{x}, t_j)\big\vert_{\mb\alpha = \mb\alpha^\star}}\br{\sum^T_{j=1}\E\brs{\mb\nabla_{\mb\alpha}^2 \mb{m}_{\mb\alpha}(\mb{x}, t_j)\big\vert_{\mb\alpha = \mb\alpha^\star}}}^{-1}. \label{eq:app:Sigmaalpha}
\end{align}
Finally, we need to define $\mb\nabla_{\mb\alpha} \mb{m}_{\mb\alpha^\star}(\mb{x}, t)$,  $\mb\nabla_{\mb\alpha}^2 \mb{m}_{\mb\alpha^\star}(\mb{x}, t)$ and $\mathrm{Var}[\mb\nabla_{\mb\alpha} \mb{m}_{\mb\alpha^\star}(\mb{x}, t_j)]$ for our case as given in \cref{eq:app:m}. The first and second derivatives for a general $\mb\alpha$ are given by 
\begin{align*}
\mb\nabla_{\mb\alpha} \mb{m}_{\mb\alpha}(\mb{x}, t) &= 2 g(t) (\mb{f} - \Eqtsmall [\mb{f}]) (\mb{f} - \Eqtsmall [\mb{f}])^\top \mb\alpha^\top (\partial_t \mb\phi(t))(\partial_t \mb\phi(t))^\top + 2 \brangle{ \partial_t g(t)(\partial_t \mb\phi(t))^\top + g(t) (\partial_t^2 \mb\phi (t))^\top, \mb{f}}, \\
\mb\nabla_{\mb\alpha}^2 \mb{m}_{\mb\alpha}(\mb{x}, t) &= 2 g(t) (\mb{f} - \Eqtsmall [\mb{f}]) (\mb{f} - \Eqtsmall [\mb{f}])^\top (\partial_t \mb\phi(t))(\partial_t \mb\phi(t))^\top.
\end{align*}

First note that $\mb\nabla_{\mb\alpha}^2 \mb{m}_{\mb\alpha}(\mb{x}, t)$ is independent of $\mb\alpha$ and therefore
\[
\mb\nabla_{\mb\alpha}^2 \mb{m}_{\mb\alpha}(\mb{x}, t)\vert_{\mb\alpha = \mb\alpha^\star} = \mb\nabla_{\mb\alpha}^2 \mb{m}_{\mb\alpha}(\mb{x}, t)
\]
for any $\mb\alpha$. Next,
\begin{align*}
\mb\nabla_{\mb\alpha} \mb{m}_{\mb\alpha}(\mb{x}, t)\vert_{\mb\alpha = \mb\alpha^\star} &= 2 g(t) (\mb{f} - \Eqtsmall [\mb{f}]) (\mb{f} - \Eqtsmall [\mb{f}])^\top {\mb\alpha^\star}^\top (\partial_t \mb\phi(t))(\partial_t \mb\phi(t))^\top + 2 \brangle{ \partial_t g(t)(\partial_t \mb\phi(t))^\top + g(t) (\partial_t^2 \mb\phi (t))^\top, \mb{f}}  \\
&= 2 \brangle{ \partial_t g(t)(\partial_t \mb\phi(t))^\top + g(t) (\partial_t^2 \mb\phi (t))^\top, \mb{f}}  ,
\end{align*}
where the final equality is due to the initial assumption of the null hypothesis that $\partialthetasmall^\star = {\mb\alpha^\star}^\top(\partial_t \mb\phi(t)) = \mb{0}$. Both of these terms are now independent of $\mb\alpha^\star$. Finally, we can work out $\mathrm{Var}[\mb{m}'_{{\mb\alpha}}(\mb{x}, t)\vert_{\mb\alpha = \mb\alpha^\star}]$ using these calculations:
\begin{align*}
    &= \Eqtsmall \brs{(2 \brangle{ \partial_t g(t)(\partial_t \mb\phi(t))^\top + g(t) (\partial_t^2 \mb\phi(t))^\top, \mb{f}} - \Eqtsmall[2 \brangle{ \partial_t g(t)(\partial_t \mb\phi(t))^\top + g(t) (\partial_t^2 \mb\phi(t))^\top, \mb{f}}])^2} \\
    &= \Eqtsmall \brs{4(\brangle{ \partial_t g(t)(\partial_t \mb\phi(t))^\top + g(t) (\partial_t^2 \mb\phi(t))^\top, \mb{f}} - \brangle{ \partial_t g(t)(\partial_t \mb\phi(t))^\top + g(t) (\partial_t^2 \mb\phi(t))^\top, \Eqtsmall[\mb{f}]})^2} \\
    &= \Eqtsmall \brs{4(\brangle{ \partial_t g(t)(\partial_t \mb\phi(t))^\top + g(t) (\partial_t^2 \mb\phi(t))^\top, \mb{f} - \Eqtsmall[\mb{f}]})^2}.
\end{align*}
Combining all these terms together gives a tractable formulation for $\mb\Sigma_{\mb\alpha}$ and hence a tractable asymptotic variance for $\sqrt{n}(\widehat{\mb\alpha} - \mb\alpha^\star)$, which does not depend on knowing $\mb\alpha^\star$.

\subsection{\texorpdfstring{Asymptotic Distribution of $\partial_t \widehat{\mb{\theta}}_t$}{Asymptotic Distribution of partial_t theta_t}}

Consider for a given $t$ taking the dot product between $\sqrt{n}(\widehat{\mb\alpha} - \mb\alpha^\star)$ and $\partial_t \mb\phi(t)$, which gives
\[
\sqrt{n} (\widehat{\mb\alpha} - \mb\alpha^\star)^\top(\partial_t \mb\phi(t)) = \sqrt{n} (\widehat{\mb\alpha}^\top (\partial_t \mb\phi(t)) - {\mb\alpha^\star}^\top (\partial_t \mb\phi(t))) = \sqrt{n} \; \widehat{\mb\alpha}^\top (\partial_t \mb\phi(t))
\]
where the final equality is due to the initial assumption of the null hypothesis, that $\partialthetasmall^\star = {\mb\alpha^\star}^\top(\partial_t \mb\phi(t)) = \mb{0}$. Then we have
\[
\sqrt{n} \; \widehat{\mb\alpha}^\top (\partial_t \mb\phi(t)) \xrightarrow{\; d \;} \mathcal{N}\br{\mb{0}, (\partial_t \mb\phi(t))^\top \mb{\Sigma}_{\mb\alpha} (\partial_t \mb\phi(t))}
\]
by the definition of multivariate Normal variables. This is the asymptotic distribution for $\partialthetasmall$.

\section{Theoretical Results of Debiased Lasso}

\subsection{Variance Estimator}
\begin{lemma}
    $|||\hat{S}(\hat{\boldsymbol{\alpha}})-\hat{S}({\boldsymbol{\alpha}}^\star)|||_\infty \leq L||\hat{\boldsymbol{\alpha}}-\boldsymbol{\alpha}^\star||_1$
where $L$ is a constant.
\end{lemma}
\begin{proof}
    on the way
\end{proof}
\begin{lemma}\label{lemma:var}
    On the event that 
    \[
    \left\|\hat{\boldsymbol{\alpha}} - \boldsymbol{\alpha}^\star \right\|_1 \leq \delta_\alpha / 2, \quad
    \left\|\tilde{\boldsymbol{\omega}}_j - \boldsymbol{\omega}_j^\star \right\|_1 \leq \delta_{\boldsymbol{\omega}}, \quad \text{and} \quad
    |||\hat{S}({\alpha}^\star) - \Sigma |||_\infty \leq \delta_\sigma / 2,
    \]
    we have 
    \begin{equation}
        \left|\hat{\sigma}^2_j - \sigma_j^2 \right| \leq (L \delta_\alpha + \delta_\sigma)\left( \left\|\boldsymbol{\omega}_j^\star \right\|^2_2 + \delta^2_{\boldsymbol{\omega}} \right) + \delta_{\boldsymbol{\omega}}^2 |||\Sigma |||_\infty
    \end{equation}
\end{lemma}

\begin{proof}
We have by definition of $\hat{\sigma}^2_j$
\begin{align}
    &\hat{\sigma}^2_j - \sigma_j^2 = \tilde{\boldsymbol{\omega}}_j^\top \hat{S}(\hat{\boldsymbol{\alpha}}) \tilde{\boldsymbol{\omega}}_j - {\boldsymbol{\omega}_j^\star}^\top \Sigma \boldsymbol{\omega}_j^\star \\
    &\implies \left|\tilde{\boldsymbol{\omega}}_j^\top \hat{S}(\hat{\boldsymbol{\alpha}}) \tilde{\boldsymbol{\omega}}_j - {\boldsymbol{\omega}_j^\star}^\top \Sigma \boldsymbol{\omega}_j^\star\right| \\
    &\leq \left|\tilde{\boldsymbol{\omega}}_j^\top \left(\hat{S}(\hat{\boldsymbol{\alpha}}) - \Sigma\right) \tilde{\boldsymbol{\omega}}_j \right| + \left|(\tilde{\boldsymbol{\omega}}_j - \boldsymbol{\omega}_j^\star)^\top \Sigma (\tilde{\boldsymbol{\omega}}_j - \boldsymbol{\omega}_j^\star)\right| \\
    &\leq |||\hat{S}(\hat{\boldsymbol{\alpha}}) - \Sigma|||_\infty \left\|\tilde{\boldsymbol{\omega}}_j\right\|^2_1 + |||\Sigma|||_\infty \left\|\tilde{\boldsymbol{\omega}}_j - \boldsymbol{\omega}_j^\star\right\|^2_1 \\
    &\leq \left(|||\hat{S}(\hat{\boldsymbol{\alpha}}) - \hat{S}(\boldsymbol{\alpha}^\star)|||_\infty + |||\hat{S}(\boldsymbol{\alpha}^\star) - \Sigma|||_\infty \right) \left\|\tilde{\boldsymbol{\omega}}_j\right\|^2_1 + |||\Sigma|||_\infty \left\|\tilde{\boldsymbol{\omega}}_j - \boldsymbol{\omega}_j^\star\right\|^2_1 \\
    &\leq \left(L\left\|\hat{\boldsymbol{\alpha}} - \boldsymbol{\alpha}^\star\right\|_1 + |||\hat{S}(\boldsymbol{\alpha}^\star) - \Sigma|||_\infty \right) \left\|\tilde{\boldsymbol{\omega}}_j\right\|^2_1 + |||\Sigma|||_\infty \left\|\tilde{\boldsymbol{\omega}}_j - \boldsymbol{\omega}_j^\star\right\|^2_1 \\
    &\leq (L\delta_{\boldsymbol{\alpha}} + \delta_\sigma) \left(\left\|\boldsymbol{\omega}_j^\star\right\|^2_1 + \delta_{\boldsymbol{\omega}}^2 \right) + |||\Sigma|||_\infty \delta_{\boldsymbol{\omega}}^2
\end{align}

as desired.
\end{proof}

\begin{lemma}\label{lemma:cov}
    There exists constants $c_0,c,c^\prime$ depend only on $M$ such that for any $t\in[c_0\sqrt{\frac{\log k}{n}},1]$ such that
    \begin{equation}
        \mathbb{P}\left(\|\hat{S}(\boldsymbol{\alpha}^\star) - \boldsymbol{\Sigma}\|_{\infty}\geq t \right)\leq c\exp\{-c^\prime t^2 n\}
    \end{equation}
\end{lemma}
\begin{proof}
    We have by denoting sample mean as $\hat{\boldsymbol{\mu}}$ and true mean as $\boldsymbol{\mu}$, we have for any $j,j^\prime\in [k]$
    \begin{align}
        &\hat{S}_{j,j^\prime}(\boldsymbol{\alpha}^\star) - \boldsymbol{\Sigma}_{j,j^\prime}= \\
        &\left(\frac{1}{n}\sum_{i=1}^n\left( [\nabla_{\boldsymbol{\alpha}}\boldsymbol{m_{\alpha}}(\boldsymbol{x}_i,t_i)]_j - \boldsymbol{\mu}_j\right)\left( [\nabla_{\boldsymbol{\alpha}}\boldsymbol{m_{\alpha}}(\boldsymbol{x}_i,t_i)]_{j^\prime} - \boldsymbol{\mu}_{j^\prime}\right) - \boldsymbol{\Sigma}_{j,j^\prime}\right) - \left(\boldsymbol{\mu}_j - \hat{\boldsymbol{\mu}}_j\right)\left(\boldsymbol{\mu}_{j^\prime} - \hat{\boldsymbol{\mu}}_{j^\prime}\right)
    \end{align}
Suppose $t$ satisfy the condition stated in lemma, and suppose 
    \begin{align}
        \left| \frac{1}{n}\sum_{i=1}^n \left([\nabla_{\boldsymbol{\alpha}}\boldsymbol{m_{\alpha}}(\boldsymbol{x}_i,t_i)]_j - \boldsymbol{\mu}_j\right)\left( [\nabla_{\boldsymbol{\alpha}}\boldsymbol{m_{\alpha}}(\boldsymbol{x}_i,t_i)]_{j^\prime} - \boldsymbol{\mu}_{j^\prime}\right)- \boldsymbol{\Sigma}_{j,j^\prime}\right| \leq t \text{            } \forall j,j^\prime \\
        \left|\hat{\boldsymbol{\mu}}_j  - \boldsymbol{\mu}_j\right| \leq t \text{            } \forall j
    \end{align}
On this event, 
    \begin{align}
        \|\hat{S}(\boldsymbol{\alpha}^\star) - \boldsymbol{\Sigma}\|_{\infty} &= \max_{j,j^\prime} \left|\hat{S}_{j,j^\prime}(\boldsymbol{\alpha}^\star) - \boldsymbol{\Sigma}_{j,j^\prime}\right|\nonumber\\
        &\leq \max_{j,j^\prime} \left| \frac{1}{n}\sum_{i=1}^n \left([\nabla_{\boldsymbol{\alpha}}\boldsymbol{m_{\alpha}}(\boldsymbol{x}_i,t_i)]_j - \boldsymbol{\mu}_j\right)\left( [\nabla_{\boldsymbol{\alpha}}\boldsymbol{m_{\alpha}}(\boldsymbol{x}_i,t_i)]_{j^\prime} - \boldsymbol{\mu}_{j^\prime}\right) - \boldsymbol{\Sigma}_{j,j^\prime} \right| + \max_{j} \left|\hat{\boldsymbol{\mu}}_j  - \boldsymbol{\mu}_j\right|^2\nonumber\\
        &\leq t+t^2 \leq 2t\nonumber
    \end{align}
By above statement, we have by boundness of random variable $\nabla_{\boldsymbol{\alpha}}\boldsymbol{m_{\alpha}}(\boldsymbol{x},t)$ and Hoffeding's inequality, there exists $c_1,c_2$ depend on $M$ only that 
\begin{align}
    \mathbb{P}\left(\left|\left([\nabla_{\boldsymbol{\alpha}}\boldsymbol{m_{\alpha}}(\boldsymbol{x}_i,t_i)]_j - \boldsymbol{\mu}_j\right)\left( [\nabla_{\boldsymbol{\alpha}}\boldsymbol{m_{\alpha}}(\boldsymbol{x}_i,t_i)]_{j^\prime} - \boldsymbol{\mu}_{j^\prime}\right)-\boldsymbol{\Sigma}_{j,j^\prime}\right| \geq t\right) &\leq 2\exp\{-c_1 t^2 n\}\\
    \mathbb{P}\left(\left|\hat{\boldsymbol{\mu}}_j  - \boldsymbol{\mu}_j\right|\geq t \right) &\leq 2\exp\{-c_2 t^2 n\}
\end{align}
Thus
\begin{equation}
   \mathbb{P}\left(\|\hat{S}(\boldsymbol{\alpha}^\star) - \boldsymbol{\Sigma}\|_{\infty}\geq t \right) \leq 2k\exp\{-c_1 t^2 n\} + 2k^2\exp\{-c_2 t^2 n\} \leq 4k^2 \exp\{-c_3 t^2 n\}\label{eq:88}
\end{equation}
for some $c_3$ depend on $M$ only. Finally we have
\begin{equation}
    \mathbb{P}\left(\|\hat{S}(\boldsymbol{\alpha}^\star) - \boldsymbol{\Sigma}\|_{\infty}\geq t \right)\leq c\exp\{-c^\prime t^2 n\}
\end{equation}
by simplifying equation (\ref{eq:88}) with bound of $t$ via choosing proper $c_0$ satisfying $c_0 > \sqrt{\frac{2}{c_3}}$.
\end{proof}

\subsection{Inverse Hessian Approximation}
\begin{lemma}[Consistency of Inverse Hessian estimator]\label{lemma:invhen}
Let $S_{{\boldsymbol{\omega}},j}$ be the support of $\boldsymbol{\omega}_j^\star$, and $s_{{\boldsymbol{\omega}},j}= |S_{{\boldsymbol{\omega}},j}|$, under condition that
\begin{equation}
    \lambda_j \geq 2\|\nabla^2_{\boldsymbol{\alpha}}\hat{J}_{\boldsymbol{\alpha}}(\boldsymbol{\alpha}^\star)\boldsymbol{\omega}^\star_j -\boldsymbol{e}_j\|_\infty
\end{equation}
we have
\begin{equation}
    \|\tilde{\boldsymbol{\omega}}_j - \boldsymbol{\omega}^\star_j\|_1 \leq \frac{6}{\kappa}s_{{\boldsymbol{\omega}},j}\lambda_j
\end{equation}

\end{lemma}
\begin{proof}
    The proof is exactly the same as proof of \cref{consi}, the only difference is we replace $\nabla_{\boldsymbol{\alpha}}\hat{J}(\boldsymbol{\alpha})$ with $\nabla_{\boldsymbol{\alpha}}\hat{J}_{\boldsymbol{\alpha}}(\boldsymbol{\alpha}^\star)\boldsymbol{\omega}^\star_j -\boldsymbol{e}_j$ and $S$ with $S_{{\boldsymbol{\omega}},j}$. So we omit the proof.
\end{proof}

\begin{lemma}
There exists constants $c_0, c,c^\prime$ depend only on $M\|\boldsymbol{\omega}_j^\star\|+1$ such that for any $t\in [c_0\sqrt{\frac{\log k}{n}},1]$, we have
\begin{equation}
      \mathbb{P}\left(\|\nabla^2_{\boldsymbol{\alpha}}\hat{J}_{\boldsymbol{\alpha}}(\boldsymbol{\alpha}^\star)\boldsymbol{\omega}^\star_j -\boldsymbol{e}_j\|_{\infty}\geq t \right) \leq c\exp\{-c^\prime t^2 n \}
\end{equation}
\label{lemma:F5}
\end{lemma}
\begin{proof}
    The result follows from fact that the random variable $\nabla^2_{\boldsymbol{\alpha}}\hat{J}_{\boldsymbol{\alpha}}(\boldsymbol{\alpha}^\star)\boldsymbol{\omega}^\star_j -\boldsymbol{e}_j$ follows sub-Gaussian distribution and therefore there exists $c_0$ such that
    \begin{equation}\label{eq:11}
        \mathbb{E}[\|\nabla^2_{\boldsymbol{\alpha}}\hat{J}_{\boldsymbol{\alpha}}(\boldsymbol{\alpha}^\star)\boldsymbol{\omega}^\star_j -\boldsymbol{e}_j\|_{\infty}] \leq c_0\sqrt{\frac{\log k}{n}}
    \end{equation}
    The proof of equation (\ref{eq:11}) is the same as \cref{lemma:Jexp}. Finally we apply Hoffeding's inequality and obtain probabilistic inequality as desired.
\end{proof}

\subsection{Gaussian Approximation Bound}\label{pf:main}
This subsection presents the proof of Gaussian Approximation Bound(GAB). Lemma \ref{lemma:A} and \ref{lemma:combo} are useful lemmas for the proof. Theorem \ref{thm:remain} talks about GAB.
\begin{lemma}\label{lemma:A}
    For $\bome \in \mathbb{R}^{k}$, let
    \begin{equation}
        A_n(\bome) = \langle \bome , \nabla_{\boldsymbol{\alpha}}\hat{J}(\boldsymbol{\alpha})\big|_{\boldsymbol{\alpha}={\boldsymbol{\alpha}}^\star}\rangle
    \end{equation}
    and
    \begin{equation}
        \sigma^2_n = \sigma_n^2(\bome) = Var[\sqrt{n}A_n(\bome)]
    \end{equation}
    Then
    \begin{equation}
        \sup_{z\in\mathbb{R}}|\mathbb{P}\{\sqrt{n}A_n(\bome)/\sigma_n \leq z\} - \Phi(z)| \leq \frac{2CM||\bome||}{\sqrt{n}\sigma_n}
    \end{equation}
    where $C = 3.3$ is a known constant.
\end{lemma}

\begin{proof}
    We have 
\begin{equation}
    \frac{\sqrt{n} A_n(\bome)}{\sigma_n} = \frac{1}{\sqrt{n}} \left\{ \sum_{i=1}^n \frac{\langle \bome, \nabla_{\boldsymbol{\alpha}} \boldsymbol{m_{\alpha}}(t_i,\boldsymbol{x}_i) \big|_{\boldsymbol{\alpha} = \boldsymbol{\alpha}^\star} \rangle}{\sigma_n} \right\}
\end{equation}
    and 
\begin{equation}
    \langle \bome, \nabla_{\boldsymbol{\alpha}} \boldsymbol{m_{\alpha}}(t_i,\boldsymbol{x}_i) \big|_{\boldsymbol{\alpha}= \boldsymbol{\alpha}^\star}  \rangle \leq \frac{2M \|\bome\|}{\sigma_n}
\end{equation}
for all $i$. Finally the Berry-Esseen inequality (Theorem 3.4 of \cite{chen2010normal}) yields
\begin{equation}
        \sup_{z\in\mathbb{R}}|\mathbb{P}\{\sqrt{n}A_n(\bome)/\sigma_n \leq z\} - \Phi(z)| \leq \frac{2CM||\bome||}{\sqrt{n}\sigma_n}
\end{equation}
where $C = 3.3$ is a known constant.
\end{proof}

\begin{lemma}(Lemma D.3 of \cite{barber2018rocket})\label{lemma:combo}
    If 
    \begin{equation}
        \sup_{z\in\mathbb{R}}|\mathbb{P}\{A\leq z\} -\Phi(z) | \leq \epsilon_A \text{ and } \mathbb{P}\{|B|\leq \delta_B, |C|\leq \delta_C \} \geq 1-\epsilon_{BC}
    \end{equation}
    for some $\epsilon_A,\epsilon_{BC},\delta_B,\delta_C \in [0,1)$, then 
    \begin{equation}
        \sup_{z\in\mathbb{R}}|\mathbb{P}\{(A+B)/(1+C)\leq z\}-\Phi(z) |\leq \delta_B + \frac{\delta_C}{1-\delta_C} + \epsilon_A + \epsilon_{BC}
    \end{equation}
\end{lemma}

\begin{theorem}{(Restatement of \cref{thm:main})}\label{thm:remain}
    For $\delta_{\boldsymbol{\alpha}}, \delta_{\boldsymbol{\omega}}, \lambda_{\boldsymbol{\alpha}}, \lambda_j, \delta_{\sigma} \in [0,1)$, define the event
    \begin{equation}
        \boldsymbol{\mathcal{E}} =
        \left\{
        \begin{array}{ll}
        2\left\|\nabla_{\boldsymbol{\alpha}}\hat{J}(\boldsymbol{\alpha}) \big|_{\boldsymbol{\alpha}={\boldsymbol{\alpha}}^\star}\right\|_\infty \leq \lambda_{\boldsymbol{\alpha}}, &
        2\left\|\nabla^2_{\boldsymbol{\alpha}}\hat{J}(\boldsymbol{\alpha}) \big|_{\boldsymbol{\alpha}={\boldsymbol{\alpha}}^\star} \boldsymbol{\omega}^\star_j - \boldsymbol{e}_j\right\|_\infty \leq \lambda_j,  
        \\
        \left\|\hat{\boldsymbol{\alpha}} - \boldsymbol{\alpha}^\star \right\|_1 \leq \delta_{\boldsymbol{\alpha}}, &
        \left\|\tilde{\boldsymbol{\omega}}_j - \boldsymbol{\omega}_j^\star \right\|_1 \leq \delta_{\boldsymbol{\omega}},
        \\
        |||\hat{S}(\hat{\boldsymbol{\alpha}}) - \hat{S}(\boldsymbol{\alpha}^\star)|||_\infty \leq \delta_\sigma / 2, &
        |||\hat{S}(\boldsymbol{\alpha}^\star) - \boldsymbol{\Sigma}|||_\infty \leq \delta_\sigma / 2
        \end{array}
        \right\}
    \end{equation}
    Suppose $\mathbb{P}(\boldsymbol{\mathcal{E}}) \geq 1 - \epsilon$. We have 
    \begin{equation}
        \sup_{z \in \mathbb{R}} \left|\mathbb{P}\left\{\frac{\sqrt{n}(\tilde{\boldsymbol{\alpha}}_j - \boldsymbol{\alpha}_j^\star)}{\hat{\sigma}_j} \leq z \right\} - \Phi(z)\right| \leq \Delta_1 + \Delta_2 + \Delta_3 + \epsilon
    \end{equation}
\end{theorem}

\begin{proof}
We have by definition of debiased lasso
\begin{align}
     &\tilde{{\ba}}_j = \hat{{\ba}}_j - \tilde{\bome}_j^\top\nabla_{\boldsymbol{\alpha}}\hat{J}(\boldsymbol{\alpha})\big|_{\boldsymbol{\alpha}=\hat{\boldsymbol{\alpha}}}
        \\
    &= \hat{{\ba}}_j - {w^\star_j}^\top\nabla_{\boldsymbol{\alpha}}\hat{J}(\boldsymbol{\alpha})\big|_{\boldsymbol{\alpha}=\hat{\boldsymbol{\alpha}}} + (\tilde{\bome}_j - \bome_j^\star)^\top\nabla_{\boldsymbol{\alpha}}\hat{J}(\boldsymbol{\alpha})\big|_{\boldsymbol{\alpha}=\hat{\boldsymbol{\alpha}}}
        \\
    & = \hat{{\ba}}_j - {\bome^\star_j}^\top\left(\nabla_{\boldsymbol{\alpha}}\hat{J}(\boldsymbol{\alpha})\big|_{\boldsymbol{\alpha}={\boldsymbol{\alpha}}^\star}+\nabla^2_{\boldsymbol{\alpha}}\hat{J}(\boldsymbol{\alpha})\big|_{\boldsymbol{\alpha}={\boldsymbol{\alpha}}^\star}(\hat{\boldsymbol{\alpha}} - \boldsymbol{\alpha}^\star)\right) + (\tilde{\bome}_j - \bome_j^\star)\nabla_{\boldsymbol{\alpha}}\hat{J}(\boldsymbol{\alpha})\big|_{\boldsymbol{\alpha}=\hat{\boldsymbol{\alpha}}}
        \\
    &\implies \tilde{{\ba}}_j - {\ba}_j^\star = \underbrace{-{\bome_j^\star}^\top\nabla_{\boldsymbol{\alpha}}\hat{J}(\boldsymbol{\alpha})\big|_{\boldsymbol{\alpha}={\boldsymbol{\alpha}}^\star}}_{A} -\underbrace{\left(\nabla^2_{\boldsymbol{\alpha}}\hat{J}(\boldsymbol{\alpha})\big|_{\boldsymbol{\alpha}={\boldsymbol{\alpha}}^\star}{\bome_j^\star}-\boldsymbol{e}_j\right)(\hat{\boldsymbol{\alpha}} - \boldsymbol{\alpha}^\star) + (\tilde{\bome}_j - \bome_j^\star)^\top\nabla_{\boldsymbol{\alpha}}\hat{J}(\boldsymbol{\alpha})\big|_{\boldsymbol{\alpha}=\hat{\boldsymbol{\alpha}}}}_{B}
\end{align}
Therefore we have by lemma \ref{lemma:A} that
\begin{equation}
    \sup_{z\in\mathbb{R}}|\mathbb{P}\{\sqrt{n}A/\sigma_n \leq z\} - \Phi(z)| \leq \frac{6.6M||\bome_j^\star||}{\sqrt{n}\sigma_j} = \Delta_1
\end{equation}
        Furthermore we have 
\begin{align}
        &B = \left(\nabla^2_{\boldsymbol{\alpha}}\hat{J}(\boldsymbol{\alpha})\big|_{\boldsymbol{\alpha}={\boldsymbol{\alpha}}^\star}{\bome_j^\star}-\boldsymbol{e}_j\right)(\hat{\boldsymbol{\alpha}} - \boldsymbol{\alpha}^\star) + (\tilde{\bome}_j - \bome_j^\star)^\top\nabla_{\boldsymbol{\alpha}}\hat{J}(\boldsymbol{\alpha})\big|_{\boldsymbol{\alpha}=\hat{\boldsymbol{\alpha}}} \\
        & = \underbrace{\left(\nabla^2_{\boldsymbol{\alpha}}\hat{J}(\boldsymbol{\alpha})\big|_{\boldsymbol{\alpha}={\boldsymbol{\alpha}}^\star}{\bome_j^\star}-\boldsymbol{e}_j\right)(\hat{\boldsymbol{\alpha}} - \boldsymbol{\alpha}^\star)}_{B_1}\\
        &+ \underbrace{(\tilde{\bome}_j - \bome_j^\star)^\top\nabla_{\boldsymbol{\alpha}}\hat{J}(\boldsymbol{\alpha})\big|_{\boldsymbol{\alpha}={\boldsymbol{\alpha}}^\star}}_{B_2} + \underbrace{(\tilde{\bome}_j - \bome_j^\star)^\top\left(\nabla_{\boldsymbol{\alpha}}\hat{J}(\boldsymbol{\alpha})\big|_{\boldsymbol{\alpha}=\hat{\boldsymbol{\alpha}}} - \nabla_{\boldsymbol{\alpha}}\hat{J}(\boldsymbol{\alpha})\big|_{\boldsymbol{\alpha}={\boldsymbol{\alpha}}^\star}\right)}_{B_{3}}
\end{align}
and by Taylor expansion
\begin{equation}
    \nabla_{\boldsymbol{\alpha}}\hat{J}(\boldsymbol{\alpha})\big|_{\boldsymbol{\alpha}=\hat{\boldsymbol{\alpha}}} - \nabla_{\boldsymbol{\alpha}}\hat{J}(\boldsymbol{\alpha})\big|_{\boldsymbol{\alpha}={\boldsymbol{\alpha}}^\star} = (\hat{\boldsymbol{\alpha}}-\boldsymbol{\alpha}^\star)\frac{{X^o}^\top G X^o}{n}
\end{equation}
Hence by Holder's inequality:
\begin{align}
    &|B_1| \leq 2 \left\|\hat{\boldsymbol{\alpha}} - \boldsymbol{\alpha}^\star \right\|_1 \left\|\nabla^2_{\boldsymbol{\alpha}} \hat{J}(\boldsymbol{\alpha}) \big|_{\boldsymbol{\alpha} = \boldsymbol{\alpha}^\star} \boldsymbol{\omega}_j^\star - e_j \right\|_\infty \leq \lambda_j \delta_{\boldsymbol{\alpha}}
    \\
    &|B_2| \leq 2 \left\|\tilde{\boldsymbol{\omega}}_j - \boldsymbol{\omega}_j^\star \right\|_1 \left\|\nabla_{\boldsymbol{\alpha}} \hat{J}(\boldsymbol{\alpha}) \big|_{\boldsymbol{\alpha} = \boldsymbol{\alpha}^\star} \right\|_\infty \leq \delta_{\boldsymbol{\omega}} \lambda_{\boldsymbol{\alpha}}
    \\
    &|B_3| \leq K \left\|\hat{\boldsymbol{\alpha}} - \boldsymbol{\alpha}^\star \right\|_1 \left\|\tilde{\boldsymbol{\omega}}_j - \boldsymbol{\omega}_j^\star \right\|_\infty \leq 4K \left\|\hat{\boldsymbol{\alpha}} - \boldsymbol{\alpha}^\star \right\|_1 \left\|\tilde{\boldsymbol{\omega}}_j - \boldsymbol{\omega}_j^\star \right\|_1 \leq K \delta_{\boldsymbol{\alpha}} \delta_{\boldsymbol{\omega}}
\end{align}

where $K = C
_f^2C_g$ is a constant and $C_f,C_g$ are bounds of $||f(x)||_2$ and $|g(t)|$ respectively, recall we assume bounded sufficient statistics. Therefore we have 
\begin{equation}
    \frac{\sqrt{n}|B|}{\sigma_j} \leq \frac{\sqrt{n}(\lambda_j \delta_{\boldsymbol{\alpha}} + \delta_{\boldsymbol{\omega}} \lambda_{\boldsymbol{\alpha}} + K \delta_{\boldsymbol{\alpha}} \delta_{\boldsymbol{\omega}})}{\sigma_j} = \Delta_2
\end{equation}

Moreover, by \cref{lemma:var},
\begin{equation}
    C = \left|\frac{\hat{\sigma}_j}{\sigma_j} - 1\right| = \left|\frac{\hat{\sigma}_j - \sigma_j}{\sigma_j}\right| 
    \leq \left|\frac{\hat{\sigma}_j^2 - \sigma_j^2}{\sigma_j^2}\right| 
    \leq \frac{(2L \delta_{\boldsymbol{\alpha}} + \delta_\sigma)\left(\|\boldsymbol{\omega}_j^\star\|^2 + \delta_{\boldsymbol{\omega}}^2\right) + \|\|\Sigma\|\|_\infty \delta_{\boldsymbol{\omega}}^2}{\sigma_j^2} = \delta_C
\end{equation}

where first inequality can be derived using the difference of squares formula.
Finally we apply \ref{lemma:combo}, obtain
\begin{equation}
        \sup_{z\in\mathbb{R}}\left|\mathbb{P}\{\sqrt{n}(\tilde{\boldsymbol{\alpha}}_j-\boldsymbol{\alpha}_j^\star)/\hat{\sigma}_j\leq z \} - \Phi(z)\right| \leq \Delta_1+\Delta_2+\Delta_3 +\epsilon
\end{equation}
where $\Delta_3 = \frac{\delta_C}{1-\delta_C}$.
\end{proof}

\subsection{Proof of Theorem \ref{thm:main2}}\label{pf:main2}

\begin{theorem}
    Let $\tilde{\boldsymbol{\alpha}}_j$ be debiased lasso estimator with tuning parameter
    \begin{equation}
        \lambda_{\boldsymbol{\alpha}} \in \mathcal{O}\left(\sqrt{\frac{\log k}{n}}\right); \text{ and }  \lambda_j \in  \mathcal{O}\left(\sqrt{s_{\boldsymbol{\omega},j} \frac{\log k}{n}}\right)
        \end{equation}
    we have there exists positive constants $c,c^\prime$ such that
    \begin{equation}
    \sup_{z\in\mathbb{R}} \left|\mathbb{P}\{\sqrt{n}(\tilde{\boldsymbol{\alpha}}_j-\boldsymbol{\alpha}_j)/\hat{\sigma}_j \leq z\}-\Phi(z)\right|\leq \mathcal{O}\left(\sqrt{n}s^{3/2}_{\boldsymbol{\omega},j} s{\frac{\log k}{n}}\right) + c\exp\{-c^\prime \log k\}
    \end{equation}
        
\end{theorem}
\begin{proof}
Consider the event $\boldsymbol{\mathcal{E}}^L $
    \begin{align}
        2||\nabla_{\boldsymbol{\alpha}}\hat{J}(\boldsymbol{\alpha}^\star)||_{\infty} &\leq \lambda_{k}  \label{eq:92}
        \\
        2||\nabla^2_{\boldsymbol{\alpha}}\hat{J}(\boldsymbol{\alpha}^\star)-\boldsymbol{e}_k||_{\infty} &\leq \lambda_{\boldsymbol{\alpha}} \label{eq:93}
        \\
        ||\hat{S}(\boldsymbol{\alpha}^\star)-\boldsymbol{\Sigma}||_{\infty}&\leq \sqrt{s}\lambda_{\boldsymbol{\alpha}}
    \end{align}
We have $\boldsymbol{\mathcal{E}}^L \subseteq \boldsymbol{\mathcal{E}}$ under \cref{ass:RE} since the following:\\
First we have by \cref{consi} that from equation (\ref{eq:92}) with \cref{ass:RE}
\begin{equation}
    \|\hat{\boldsymbol{\alpha}}-\boldsymbol{\alpha}^\star\|_1 \leq \frac{6}{\kappa}\lambda_{\boldsymbol{\alpha}}s \in \mathcal{O}\left(s\sqrt{\frac{\log k}{n}}\right)
\end{equation}
In addition, we have from \cref{lemma:invhen} that from equation (\ref{eq:93})
\begin{equation}
    \|\tilde{\boldsymbol{\omega}}_j-\boldsymbol{\omega}^\star_j\|_1 \leq \frac{6}{\kappa}\lambda_{j}s_{\boldsymbol{\omega},j}\in\mathcal{O}\left(\sqrt{s_{\boldsymbol{\omega},j}^3 \frac{\log k}{n}}  \right)\label{eq:delta2O}
\end{equation}
therefore $\boldsymbol{\mathcal{E}}^L \in \boldsymbol{\mathcal{E}}$ and we have 
\begin{equation}
    \Delta_2 \in \mathcal{O}\left(\sqrt{n}s^{3/2}_{\boldsymbol{\omega},j} s{\frac{\log k}{n}}\right)
\end{equation}
We ignore $\Delta_1$ and $\Delta_3$ since they are of smaller order.\\
Next we bound $\mathbb{P}\left(\boldsymbol{\mathcal{E}}^{L,c}\right)$. Let
\begin{align}
    \boldsymbol{\mathcal{E}}_1 &= \{2||\nabla_{\boldsymbol{\alpha}}\hat{J}(\boldsymbol{\alpha}^\star)||_{\infty} \leq \lambda_{k}\}\\
    \boldsymbol{\mathcal{E}}_2 &= \{2||\nabla^2_{\boldsymbol{\alpha}}\hat{J}(\boldsymbol{\alpha}^\star)-\boldsymbol{e}_k||_{\infty} \leq \lambda_{\boldsymbol{\alpha}}\}\\
    \boldsymbol{\mathcal{E}}_3 &= \{||\hat{S}(\boldsymbol{\alpha}^\star)-\boldsymbol{\Sigma}||_{\infty}\leq \sqrt{s}\lambda_{\boldsymbol{\alpha}}\}\\
\end{align}
It is obvious that 
\begin{equation}
    \mathbb{P}\left(\boldsymbol{\{{\mathcal{E}}^{L}}\}^c\right)\leq \sum_{i=1}^3  \mathbb{P}\left(\boldsymbol{\mathcal{E}}^{c}_i\right)
\end{equation}
Under bounded condition, we have the following:
By \cref{lemma:Jexp} and \cref{lemma:F5}, there exist constants \(c_1\), \(c_1^\prime\), \(c_2\), and \(c_2^\prime\).
\begin{align}
    \mathbb{P}\left(\boldsymbol{\mathcal{E}}^{c}_1\right) &= \mathbb{P}\left(2||\nabla_{\boldsymbol{\alpha}}\hat{J}(\boldsymbol{\alpha}^\star)||_{\infty} > \lambda_{k}\right)\leq c_1\exp\{-c_1^\prime\log k\}\\
    \mathbb{P}\left(\boldsymbol{\mathcal{E}}^{c}_2\right) &= \mathbb{P}\left(2||\nabla^2_{\boldsymbol{\alpha}}\hat{J}(\boldsymbol{\alpha}^\star)-\boldsymbol{e}_k||_{\infty} > \lambda_{\boldsymbol{\alpha}}\right)\leq c_2\exp\{-c_2^\prime\log k\}
\end{align}
and by \cref{lemma:cov} there exists $c_3,c_3^\prime$
\begin{equation}
     \mathbb{P}\left(\boldsymbol{\mathcal{E}}^{c}_3\right) = \mathbb{P}\left(||\hat{S}(\boldsymbol{\alpha}^\star)-\boldsymbol{\Sigma}||_{\infty}> \sqrt{s}\lambda_{\boldsymbol{\alpha}}\right)\leq c_3\exp\{-c_3^\prime\log k\}\label{eq:107}
\end{equation}
Therefore there exists $c,c^\prime$
\begin{equation}
     \mathbb{P}\left(\boldsymbol{\{{\mathcal{E}}^{L}}\}^c\right) \leq c\exp\{-c^\prime \log k\}
\end{equation}
Finally we complete the proof with combining the bounds of (\ref{eq:107}) and (\ref{eq:delta2O}),
\begin{equation}
    \sup_{z\in\mathbb{R}} \left|\mathbb{P}\{\sqrt{n}(\tilde{\boldsymbol{\alpha}}_j-\boldsymbol{\alpha}_j)/\hat{\sigma}_j \leq z\}-\Phi(z)\right|\leq \mathcal{O}\left(\sqrt{n}s^{3/2}_{\boldsymbol{\omega},j} s{\frac{\log k}{n}}\right) + c\exp\{-c^\prime \log k\}
\end{equation}
\end{proof}

\section{Extra Changepoint Algorithm Details} \label{app:changepoint}

\cref{sec:practical:thresholding} describes our approach to changepoint detection, given the asymptotic distribution of our estimator. Our detector depends on a significance level $\delta > 0$. Smaller values of $\delta$ (e.g. $\delta = 0.01$) are likely to produce fewer false positives but risk not detecting the full period of change, whereas larger values (e.g. $\delta = 0.05$) will produce more false positives but will not risk losing potential true change periods. There is a trade-off between smaller and larger values of $\delta$, which is standard in hypothesis testing. Choice of $\delta$ is up to the practitioner. In either case, we propose two additional frameworks to reduce the chance of false positives in the detection algorithm.

\paragraph{Small-peak criterion} Setting the significance level $\delta$ means that there is a $1-\delta$ probability that the detector will exceed the threshold by pure chance. We propose to also disregard any change period $\Delta$ if 
\[
\max_{t} \Delta - \min_{t} \Delta < \varepsilon_{\text{SP}},
\]
i.e. the total amount of time in the change period is less than $\varepsilon_{\text{SP}}$. Alternatively, this condition could be written as $|\Delta| < \varepsilon_{\text{SP}} T$. 

\paragraph{Peak-proximity criterion} We also implement an adapted version of the $\varepsilon$-criterion, as described in \citet{rmosum}. Given two periods of change $\Delta_1$ and $\Delta_2$ for which $t_1 \in \Delta_1$ and $t_2 \in \Delta_2$, this criterion classifies the two periods of change as the same period if
\[
\min_{\substack{t_1 \in \Delta_1 \\ t_2 \in \Delta_2}} | t_1 - t_2 | < \varepsilon_{\text{PP}},
\]
i.e. the smallest difference between change period is less than $\varepsilon_{\text{PP}}$.

Choice of $\varepsilon_{\text{SP}}$ and $\varepsilon_{\text{PP}}$ depend greatly on the application. For example, for smaller $\delta$, we recommend also choosing smaller $\varepsilon_{\text{SP}}$ as one is less likely to observe false positives. Additionally, if changepoints are expected to be close together, we recommend smaller values of $\varepsilon_{\text{PP}}$ to avoid mis-classifying two changepoints as one. 

Throughout most of our experiments, we use $\varepsilon_{\text{SP}} = 0.01$ and $\varepsilon_{\text{PP}} = 0.02$ for significance level $\delta = 0.01$, with two exceptions. In our benchmarks in \cref{sec:benchmark}, we expect fewer changepoints to be in close proximity, and therefore increase these values by a small amount, $0.05$ each, and use $\varepsilon_0 = 0.015$ and $\varepsilon_1 = 0.025$. \cref{sec:applications:gfc} contains three visually distinct changepoints, but the latter two changes would be misclassified as the same changepoint if $\varepsilon_{\text{PP}} = 0.02$. Using $\varepsilon_{\text{PP}} = 0.01$ successfully allows the method to detect these as distinct changes. In this case, these two changepoints are clearly visually separate from one another, and further, $\partialthetahatsmall$ has a different sign for each change, highlighting that they are distinct.

\section{Benchmark Details for \cref{sec:benchmark}} \label{app:benchmark_details}

Tables \ref{tab:benchmark_abrupt} and \ref{tab:benchmark_pwl} give experimental results for two distinct changepoint detection experiments. The first experiment is time series data generated with abrupt changes in the mean, variance, and mean and variance. The second containing smooth changes in the mean, variance, and mean and variance over a longer time period. Here we detail the experiment setups and the methods used in the tables.

\subsection{Abrupt Change Benchmark (\cref{tab:benchmark_abrupt})}

The three experiments used to benchmark the methods for changepoint detection in \cref{tab:benchmark_abrupt} are:
\begin{itemize}
    \item \textbf{Mean} change experiment: The time series is Gaussian noise with mean $\mu(t)$ which is piecewise constant, with fixed $\sigma^2=1$. A changepoint at $t=0.5$ shifts the mean from $\mu(t)=0$ to $\mu(t) = 2$.
    \item \textbf{Variance} change experiment: The time series is Gaussian noise with variance $\sigma^2_t$ which is piecewise constant, with fixed $\mu=0$. A changepoint at $t=0.5$ shifts the variance from $\sigma(t)^2=1$ to $\sigma(t)^2 = 3$.
    \item Mean \& Variance (\textbf{Both}) change experiment: The time series is Gaussian noise with mean $\mu(t)$ and variance $\sigma^2_t$, both piecewise constant. A changepoint at $t=0.33$ shifts the mean from $\mu(t) = 0$ to $\mu(t) = 2$, and a further changepoint at $t=0.66$ shifts the variance from $\sigma(t)^2=1$ to $\sigma(t)^2 = 3$.
\end{itemize}

For each experiment, the full time series was generated with length $T=5000$. When running our method, we binned this time series into $n=5$ intervals so that the re-labelled time series had new length $1000$. Other methods used for comparison used the original, un-binned time series data.

We implement MOSUM, \citep{mosum, rmosum} using the \texttt{mosum} package in python \citep{pypi-mosum}. For all MOSUM methods, we use bandwidth $G=T/6$ based on several factors. The first is that across simulations, we found this to be a well performing bandwidth. Secondly, the experiments considered in these experiments do not have close together changes, and we do not need a smaller bandwidth to cover that. Whilst the choice of bandwidth is important, we considered multiple options as different fractions of the time series length, and settled on this value as the consistently best performing one for experiments. For a more comprehensive overview of bandwidth selection, see \citet{kirch2022}. 

To detect changes in the variance using MOSUM (called MOSUM (var) in the table), we transform the time series $\{\mb{x}_i\}^T_{i=1}$ as follows
\begin{equation}
\widehat{\mb{x}}_i = \br{\mb{x}_i- \frac{1}{T}\sum^T_{i=1}\mb{x}_i }^2
\label{eq:mosumvar}
\end{equation}
for all $i = 1, \dots, T$, where $T$ is the length of the time series. Then we apply MOSUM for mean-change detection on $\{\widehat{\mb{x}_i}\}^T_{i=1}$.

To detect changes in both mean and variance (called MOSUM (comb.) in the table) is a combination of MOSUM for mean change detection and variance change detection. We run both MOSUM variations on the time series and combine the results afterwards.

We use PELT \citep{pelt} with the RBF cost function for both mean and variance changes. The penalty on the number of changepoints we use is given by $2\log T$. We implement PELT with the \texttt{ruptures} package, see \citet{ruptures} for details.

For our method, TSM-DE (RBF) and TSM-DE (SWL), we choose hyperparameters with cross-validation, and detect changepoints using \cref{eq:CP}.

\subsection{Piecewise Linear Change Benchmark (\cref{tab:benchmark_pwl})}

We perform a similar experiment to the abrupt change benchmark, but instead of parameters changing suddenly at fixed changepoints, they change gradually over a given time period.

\begin{itemize}
    \item \textbf{Mean} change experiment: The time series is Gaussian noise with mean $\mu(t)$ given by 
    \[
    \mu(t) = \begin{cases}
        0             & \text{ if } t < 1/3, \\ 
        10(t - 1/3)   & \text{ if } 1/3 \leq t < 2/3, \\
        10/3          & \text{ if } t \geq 1/3,        
    \end{cases}
    \]
    i.e. the `middle section', where $1/3 \leq t < 2/3$ is the smooth change. In this case, $\sigma^2 = 1$ is constant.
    \item \textbf{Variance} change experiment: The time series is Gaussian noise with variance $\sigma(t)$ given by
    \[
    \sigma(t) = \begin{cases}
    1             & \text{ if } t < 1/3, \\ 
    6t - 1        & \text{ if } 1/3 \leq t < 2/3, \\
    3             & \text{ if } t \geq 1/3.    
    \end{cases}
    \]
    In this case $\mu = 0$ is constant.
    \item Mean \& Variance (\textbf{Both}) change experiment: The time series is Gaussian noise with $\mu(t)$ and $\sigma(t)$ given by
    \[
    \mu(t) = \begin{cases}
        0             & \text{ if } t < 1/5, \\ 
        10(t - 1/5)   & \text{ if } 1/5 \leq t < 2/5, \\
        2          & \text{ if } t \geq 2/5,        
    \end{cases} \qquad
    \sigma(t) = \begin{cases}
    1             & \text{ if } t < 3/5, \\ 
    10t - 5        & \text{ if } 3/5 \leq t < 4/5, \\
    3             & \text{ if } t \geq 4/5.    
    \end{cases}
    \]
\end{itemize}

Similar to the abrupt experiment, the full time series was generated with length $T=5000$ which was binned into $n=5$ intervals for the TSM-DE methods. Other methods used for comparison used the original, un-binned time series data.

We implement the Piecewise Linear MOSUM (called PWL MOSUM in the table) method described by \citet{kim2024} for comparison, using the R implementation also provided by the authors. For this method, we use the authors recommendation of multiple bandwidths as described in \citet{kim2024}. Similar to MOSUM in the abrupt changepoint experiment above, we transform the time series according to \cref{eq:mosumvar} to detect changes in variance. To detect changes in both the mean and variance (called PWL MOSUM (comb.) in the table), we apply the method to mean changes and variance changes separately and combine the results afterwards.

For our method, TSM-DE (RBF) and TSM-DE (SWL), we choose hyperparameters with cross-validation, and detect entire change periods using \cref{eq:CR}. The `changepoints' that we detect, for which we calculate the covering metric values from, are the boundaries (i.e. beginning and end) of the change period(s) detected.

\section{Hyperparameter Selection} \label{app:hyperparam} 

Depending on the experiment, and model for $\partial_t \mb\theta_t$, there are a few hyperparameters that must be chosen for the TSM-DE method. These are 
\begin{itemize}
    \item $\ell_1$-regularisation parameter $\lambda$.
    \item Nadarya-Watson estimator kernel and kernel hyperparameters. We always use a Gaussian kernel for the weighted expectation, which requires one bandwidth hyperparameter.
    \item For the \textit{RBF time feature} (see \cref{sec:modelling:rbf}), the number of basis functions $b$, and kernel bandwidth parameter. 
    \item For the \textit{sliding window linear model} (see \cref{sec:modelling:ll}), the window size $w$.
\end{itemize}

Provided that $n > 1$ (and if $n=1$, then we can apply the binning approach described in \cref{sec:practical:expectation}), we construct a validation set that spans all time points of size $n_{\text{val}} < n$ at each time point. Then, we perform a grid search over a specified set of hyperparameters, and choose those hyperparameters that minimise the testing loss, which is calculated on the sample objective, given in \cref{eq:sampleobj}, which is un-penalised ($\lambda = 0$) and contains no weighted expectation via the Nadarya-Watson estimator.

We can repeat this process multiple times until all samples are covered, which corresponds to cross-validation, or use a single validation set only.
